# Supplementary material for: Adapting Behaviors via Reactive Synthesis
Source: arXiv:2105.13837 source file (2021-05-28)
Supplement: Supplementary file 1 [file AppendixExperiments.tex]

\section{Experiments Supplemental}\label{app:Experiments}

%The {\em motivating example}\dftodo{come up with a better name} is parameterized in the number of variables controlled by the target and adaptee systems (also called the number of bits). For a parameter $n>0$, let the target system control the variables $\mathcal T=\{t_1,\dots,t_n\}$, and the adaptee system control the variables $\mathcal A=\{a_1,\dots,a_n\}$. Let $t_v$ (or $a_v$) denote the state over $\mathcal T$ (or $\mathcal A$)  that encodes the number $v\in\mathbb{N}$ in binary. The target transitions are of the form $(t_0,t_i)$ and $(t_i,t_i)$, where $i\in\{1,n\}$.  The adaptee transitions are of the form $(a_0,a_{2i+1})$, $(a_{2i},a_{2i+1})$, $(a_{2i+1},a_{2i})$ for $i \in \{1,\lfloor (n-1)/2 \rfloor\}$ and $(a_1,a_0)$. The details for $n=2$ has been shown in Section~\ref{sec:transducers}. Clearly, in a scenario with $n$ bits, the specification consists of $2n$ variables. We generate 10 such benchmarks with $n\in\{1,\ldots,10\}$.

\begin{table}[t!]
    \centering
    \begin{tabular}{|c|c||c|c|c|c|c|c|c|c|c|c|}
    \hline
         \multicolumn{2}{|c||}{$n$} & 1 & 2 & 3 & 4 & 5 & 6 & 7 & 8 & 9 & 10   \\ \hline \hline

        \multirow{2}{*}{$\sf{MultiMode(\text{$n$})}$} & \tool{} & 0.06 & 0.05 & 0.05 & 0.06 & 0.06 & 0.08 & 0.1 & 0.19 & 0.46 & 1.07 \\
         \cline{2-12}
         & Strix & 0.13 & 0.29 & TO & TO & TO & TO & TO & TO & TO & TO \\ \hline \hline

         \multirow{2}{*}{$\sf{Cleaning(\text{$n$})}$} & \tool{} & 0.05 & 0.05 & 0.07 & 0.09 & 0.16 & 0.26 & 0.63 & 1.16 & 1.78 & 2.43 \\
         \cline{2-12}
         & Strix & 0.31 & 0.75 & 58.3 & TO & TO & TO & TO & TO & TO & TO \\
         \hline
         
         \hline \hline
         
        \multirow{2}{*}{$\sf{Railways(\text{$n,2$})}$} & \tool{} & - & 0.11 & 0.17 & 0.71 & 3.88 & 11.8 & 15.1 & 40.8 & 219 & TO  \\
         \cline{2-12}
         & Strix & - & 382 & TO & TO & TO & TO & TO & TO & TO & TO \\
         \hline
         
        \multirow{2}{*}{$\sf{Railways(\text{$n,3$})}$} & \tool{} & - & 0.07 & 0.36 & 1.67 & 8.39 & 29.8 & 50.3 & 102 & TO & TO \\
         \cline{2-12}
         & Strix & - & 381 & TO & TO & TO & TO & TO & TO & TO & TO \\
         \hline

    \end{tabular}
    
    \caption{Mean realizability check running times (sec.)}
    \label{tbl:results}
\end{table}

\begin{figure}

 %\hfill 
  % \begin{subfigure}{0.5\textwidth}
        \centering
        \includegraphics[width=0.5\textwidth]{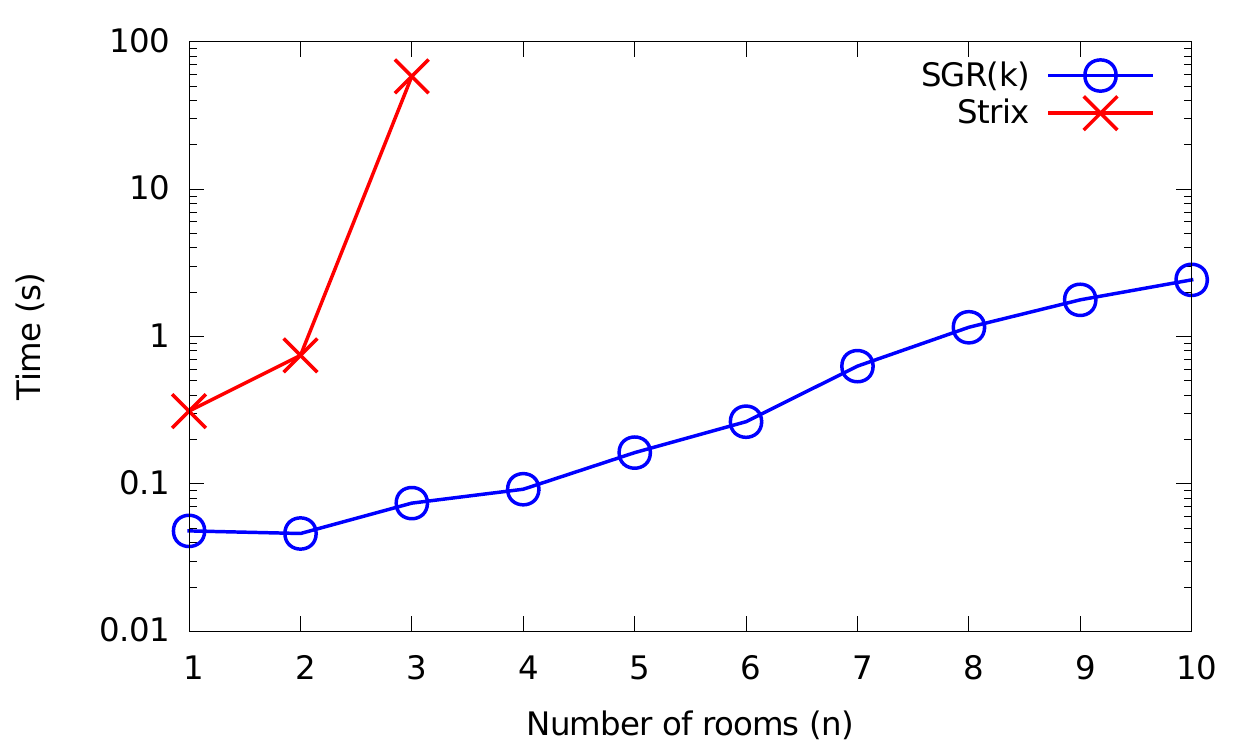}
       \caption{Mean Cleaning Robots running time \label{fig:robots}} 
%    \end{subfigure}
%    \hfill
\end{figure}

%Table~\ref{tbl:results} presents mean running time results obtained for each specification and each tool (in sec.). The table rows refer to the benchmarks we examine, and the columns refer to the value of the parameter $n$. As an example, for the specification $\sf{Cleaning(\text{3})}$, \tool{}'s mean running time is 0.07 sec. (row titled $\sf{Cleaning(\text{n})}$;\tool{}, column titled 3) and $\mathsf{Strix}$'s median realizability check running time is 58.3 sec. (row titled $\sf{Cleaning(\text{n})}$;Strix), column titled 4). Cells reading `TO' indicate experiments reached a timeout. 

%Figure~\ref{fig:robots} shows a plot for the Cleaning Robots benchmark mean running times.
