# Supplementary material for: Adapting Behaviors via Reactive Synthesis
Source: arXiv:2105.13837 source file (2021-05-28)
Supplement: Supplementary file 2 [file OldAppendixExamples.tex]

\section{Examples}


% 

Reactive systems are systems that interact with the environment through an on going input/output process reactions in which the system responds to the triggers emitted by the environment.
For such systems, there is typically a system specification formalized in some logic, that describes the exact input/output reactions that the system should act upon. Reactive synthesis, is then the process of constructing such system from it's given specification.

While reactive synthesis specification reasons about the interaction between the actions of the system and the environment, sometimes focusing on the action is to delicate for the specifier, and the required reasoning level is more high-level in which the specification reason on the relationship between the systems and the environment \textit{behaviors}, where the specifier is less interested in the exact action-level implementation detail, but rather just have the system's behavior to some environment specific behaviors that may occur. The environment, in that sense, can be the world, or another system that the original system needs to react to, or perhaps even just a system which the original system wants to imitate, under certain restrictions.
We give examples.

\begin{enumerate}
\item \textbf{Transmitter station.} Consider an intermediate transmitter station (called System $B$) that receives transmission from a the main distributer unit (called System $A$) and then sends the transmissions to a receiver unit. Due to certain constraints (e.g. limited bandwith of the transmitter station, handling many distributer stations), the transmitter station adjusts the transmissions before sending them to the receiver. While doing so, however, certain properties of the 
original transmission are to be maintained. For example, some transmissions may have urgency sense in them, while other more relaxed. It is then natural for the designer of the transmitter station to specify the required behavior of the transmitter for every type of behavior received by the distributer.

\item \textbf{Systems modification} Consider an original system $A$ that is running a set of specific scenarios, each is a sequence of actions. The designer wishes to build a system $C$, but to use system $A$ in a black-box manner. Therefore the designer constructs System $C$ by taking system $C$, with an additional \textit{wrapper} (called System $B$) that is needed to be synthesized. The specification for the wrapper then naturally designed as required behavior adjustment, rather than for every specific action. For example,  
the designer may try to build a system $C$ that imitates the behavior of System $A$ as much as possible under the restriction that system $C$ has additional behavioral constraints which the designer should consider. Note that in this example, there is no actual reactivity between System $A$ and the wrapper: the wrapper observes the behavior of System $A$ and adjust it to meet the overall specification that the designer has specified.

\item \textbf{Traffic Controller.}
As another example of behavior control, consider the following example given from Shield Synthesis \cite{}.
Assume we have a controller for a traffic light at an intersection (let's call this controller $System A$).
We'll call the output of this controller a and assign it one of four values: $rr$, $rg$, $gr$ and $gg$, which indicate for each of the two lights whether that light is red ($r$) or green ($g$). The problem is that we have no guarantees about the behavior of this controller. In particular, there are two guarantees that we want to ensure: the two lights don't turn green at the same time, and the lights don't switch from $rg$ to $gr$ or vice-versa without passing through $rr$ in between. The solution in ~\cite{} is to add a \textit{shield} (which we refer to as System $B$) between the controller and the actual traffic lights. This shield takes the output a of the controller as input and outputs a new signal $b$. If $A$ would at any point violate our guarantees, System $B$ alters the output to something that would satisfy $A$. Ideally, we would also like to change the output as little as possible.
\end{enumerate}


The examples above demonstrate a large variety of problems that can be thoughts as "synthesis of behaviors" [[DF: does such term exists already?]].
Towards formalizing these example into computational models, we choose to use Linear Temporal Logic (LTL), commonly used to describe specifications for reactive synthesis \cite{}. In our setting however the specifications must not be written as general LTL formula, but take a specific form that we can use for our advantage. [[DF: I am not happy with the order of telling, we'll discuss]].
Indeed, such specification can take a special form of a collection of assume-guarantee constraints in a form of $\phi\rightarrow\psi$. However while every "assume" constraint $\phi$ is an LTL formula of the environment variables only, Every $\psi$ "guarantee" constraint is an LTL formula over system variables \textit{only}.
Note that this setting is different than the typical assume-guarantee constraints in which the "guarantee" constraints are set over both environment and system variables. 

For example, in the \textit{Transmitter station} problem, let $\{r\}$ be the alphabet of the transmissions System $A$ (the transmitter station) receives, and let $\{r'\}$ be the alphabet of the transmissions System $A$ (the transmitter station) sends. Then an example of a specification can be thought as a conjunction of constraints:

\begin{itemize}
\item $A$ is urgent, and $B$ has to address the urgency in some specific way:
$$ G(\neg r r)\rightarrow (FG((\neg r)^3r \vee (\neg r)^2 r \vee (\neg r)r)$$
(here $x^k$ means $x$ is repeated $k$ times)
\item $A$ is suspiciously relaxed:
$$GF((\neg r)^5 \wedge GF(\neg r r) \rightarrow (FG((\neg r)^8r U \neg r r))$$
\item Else $\rightarrow FG((\neg r)^3 r)$
\end{itemize}


Or as another example in the \textit{Traffic Controller} example, the specification can be thought of as a conjunction of the following constraints.

\begin{itemize}
    \item $GF(a= rr)\rightarrow GF(b=rr)$
    \item $GF(a= rg)\rightarrow GF(b=rg)$
    \item $GF(a= gr)\rightarrow GF(b=gr)$
    \item $true\rightarrow G(\neg (b=gg))$
    \item $true\rightarrow (G(X(b=gr))\rightarrow (\neg b=rg)$
    \item $true\rightarrow (G(X(b=rg))\rightarrow (\neg b=gr)$
\end{itemize}

We note that in these examples, an advantage of writing specifications as in this way, is the comfort in writing such specifications that describe behavior, as well as the readability of such terms. This was also noted in the $GR(k)$ formulation \cite{} [[DF: how are we compared to that?]].
Another advantage that we next show however, is that for certain settings there is also an efficiency advantage in solving such techniques.


\vspace{2mm}

We next discuss our technical advantages. [[DF: this shoud be expanded much further]]

\begin{itemize}
\item We show that for LTL assume and guarantee formulas that can be captured as a DBA, there is a techinque that is complexity-wise more efficient than the state-of-art techniques. Indeed, our methods is invoked on the so called delay property. that we explain in details and use. Note that DBA can use a variety of specification (such as all the examples above) as also noted in \cite{}.

\item We start by giving an explicit description of our technique, following by a symbolic description.

\item Since delay property can be thought of a special case of asynchrony between the environment and the system, we also discuss this relation.

\item Finally, we build our tool which makes use of this technique and we compare it to standard LTL synthesis approaches to see the gain of our delay technique.
\end{itemize}


% In our systems Assumptions only on the environment, and the guarantee are only on the system.

% Motivation - which system have these properties



% Add restrictions 



% Streetlights

% tic tac toe

% reduction between systems.

% Technical - what can we syntehsize.

% LTL synthesis in general 

% In some cases we offer a procedure that is highly efficient 


% %




% %




% %

% On going example:

% Street lights

% Tic Tac Toe
