# Supplementary material for: Adapting Behaviors via Reactive Synthesis
Source: arXiv:2105.13837 source file (2021-05-28)
Supplement: Supplementary file 3 [file OldAppendixGalIntro.tex]

\section{Introduction - Detailed Examples}
\label{app:introC}

The field of reactive synthesis has produced various techniques for automatic generation of  controllers that react to inputs under given constraints in a way that satisfies required specifications. These techniques have been shown to be practical in providing effective tools for the design of correct-by-construction systems.
In this paper we propose a reactive synthesis usage that resembles the  the well known adapter design pattern~\cite{gamma1995design}.

In the adapter design approach, the programmer implements a \emph{Target} interface by writing a code for an \emph{Adapter} that calls existing methods of an \emph{Adaptee} interface. For illustration, consider a class that rotates a Rubik cube and thus implements the methods {\sf rot\_left}, {\sf rot\_right}, {\sf rot\_up}, {\sf rot\_down}. Now, assume that we have a broken cube that cannot be rotated to the left. Hence, we implement {\sf broken\_rot\_left} by calling {\sf rot\_right} three times. In this example, the interface for the correct cube is the existing \emph{Adaptee} code, the code that activates it is the \emph{Adapter}, and their composition is the \emph{Target} class that implements the target interface. In this case, the pattern allows to easily overcome hardware limitations.   

In the reactive interpretation we propose, we assume an existing \emph{Adaptee} transducer that, when used, produces a stream of (input) valuations. We aim to synthesize an \emph{Adapter} that reads those inputs in run-time, and responds with (output) valuations. The \emph{Target} specification we consider for the construction of the Adapter consists of safety limitations over the steps the adapter transducer may take, and further connections between the behaviors of the adaptee and the adapter transducers. 

For illustration, assume that we have an adaptee transducer that rotates a Rubik cube. We wish to construct an adapter transducer that tracks a Rubik cube usage, and accordingly rotates a broken Rubik cube that cannot be rotated to the left. We require (e.g.) that if the green face is solved in the correct cube, then it is solved also in the broken cube. 
Note that such a transducer can be constructed by copying the rotations of the correct cube, while rotating the broken cube three times to the right upon each rotation to the left of the correct cube. This, however, in contrast to our approach, requires an infinite memory.

Therefore, we propose the following synthesis problem: given a  transducer $Adaptee$, synthesize transducer $Adapter$ such that
\[   \mathit{Adapter} \circ  \mathit{Adaptee}  \models \mathit{Target \ Specification},\]
where $\circ$ represents transducer composition. To obtain a better understanding, we provide an explicit toy example, depicted in Figure~\ref{fig:example}. The existing Adaptee transducer controls variables $t_1$ and $t_2$, and it chooses to turn on only one of them. The Adapter transducer we aim to construct controls $a_1$ and $a_2$, and it has the following limitations: if it chooses to turn on $a_1$, it cannot change the values of $a_1$ and $a_2$ anymore. But, if it turns on $a_2$, it must turn it off immediately afterwards. This \emph{safety} limitations are depicted through what we call the \emph{output} transition system. In addition to this safety property, the liveness property the composition need to satisfy is captured by the LTL, specifically GR($k$), formula: $(\ltlG \ltlF(t_1)\rightarrow \ltlG \ltlF(a_1)) \wedge (\ltlG \ltlF(t_2) \rightarrow \ltlG \ltlF(a_2))$. The output system and the GR($k$) formula constitute the target specification. We provide in Figure~\ref{fig:example} an Adapter transducer that achieves the required.





%While most of the work on software synthesis focuses on synthesizing complete systems from their specifications, our focus is on using reactive synthesis for reusing existing components. The $Adapter$ transducer can model, for example, a standard Rubik cube and the $Adaptee$ can model a Rubik cube with some hardware failure. Since we know how to operate the normal cube, we could use an $Adapter$ that translates commands that we planed to send to the normal cube to commands that we can send to faulty one. The equivalence relation can say, for example, that if a side of the normal cube would have been completed infinitely often in the expected run of the normal cube it should also be completed infinitely often in the generated run of the faulty cube.


%Generally, synthesizing a transducer is complicated - complexity wise. Indeed, Even when equality is required, synthesizing is a non trivial task. \dftodo{write much better and explain the hardness, as a step towards GRk}


%\dftodo{Now we mention GR(k) and how to utilize GR(k) that balance between expressiveness and efficiency. Mention the term "reactive synthesis".}


%To allow direct use of the language of reactive synthesis, and to allow more generality, the input to our synthesis algorithm and to the tool that implements it is a representation of $Adpatee$ and $Target$  as transition systems, as depicted in Figure~\ref{fig:example}. The $Input$ transition is a representation of the $Target$ and the $Output$ transition system is a representation of the $Adatpee$ where we ignore the inputs to the systems and the state and consider only their outputs.

\begin{figure}
    \centering
    \begin{tikzpicture}[->,>=stealth',shorten >=1pt,auto,node distance=1cm,initial text=,
      thick,node/.style={fill=blue!20,draw,
      font=\sffamily\footnotesize,minimum width=15mm}]

    \node[initial,node] (00) {$\neg t_1  \wedge \neg t_2$};
    \node[node] (01) [above of=00] {$\neg t_1  \wedge t_2$};
    \node[node] (10) [below of=00] {$t_1  \wedge \neg t_2$};
    \node [above= 0.2 cm of 01] {Adaptee (Input)};

    \draw [->] (00) --  (01);
    \draw [->] (00) --  (10);
    \draw [->] (01) edge [loop left] (01);
    \draw [->] (10) edge [loop left] (10);

    \node[initial,node] (_00) [right=2cm of 00] {$\neg a_1  \wedge \neg a_2$};
    \node[node] (_01) [above of=_00]    {$\neg a_1  \wedge a_2$};
    \node[node] (_10) [below of=_00]    {$a_1  \wedge \neg a_2$};
    \node [above= 0.2 cm of _01] {Output};

    \draw [->] (_00) edge [bend right]  (_01);
    \draw [->] (_00) --  (_10);
    \draw [->] (_01) edge [bend right]  (_00);
    \draw [->] (_10) edge [loop left] (_10);
     

    
    \node [above= 15pt of 00] {Adapter};
    
    
    
    \node[node,circle,minimum width=0mm] (0n) [below=2cm of 10] {$s_0$};
    
    
    \node[initial,circle,node,minimum width=0mm] (In) [left=2.5cm of 0n] {$ini$};
    

    

    
    \node[node,circle,minimum width=0mm] (1n) [right=3cm of 0n] {$s_1$};
    


    \draw [->] (In) edge 
            node [above,text width=2cm ]      {$\mathit{true}|\neg a_1\wedge \neg a_2$}     (0n);    
    
    \draw [->] (0n) edge [bend left] 
            node [above,text width=2cm ] (A)     {$\neg t_1|\neg a_1 \wedge a_2$}     (1n);
    
    \draw [->] (1n) edge [bend left] 
            node [below,text width=1cm ]{$\mathit{true|\neg a_1\wedge\neg a_2}$} (0n);
            
  %  \draw [->] (0n) edge [bend right] 
  %          node [left,text width=1cm ]      {$t_1 \wedge \neg t_2$}     (2n);
    
        \draw [->] (0n) edge [loop below] 
            node [below,text width=2cm ]{$t_1|a_1\wedge \neg a_2$} (0n);
    
    
    \end{tikzpicture}
    \caption{An example of an adpatee and adapter transducers. The adapter respects the output limitations, and the composition of the adaptee with the adaptor satisfies $(\ltlG \ltlF(t_1)\rightarrow \ltlG \ltlF(a_1)) \wedge (\ltlG \ltlF(t_2) \rightarrow \ltlG \ltlF(a_2))$}
    \label{fig:example}
\end{figure}

\ganote{here we proceed to talk about variable separation, GR(k), DBA, time complexity and so on. We are pretty much aligned on that part so I will stop here}

%From this point on, we will only talk about this representation of the problem, i.e., we will synthesize a controller that reads a run  of an input transition system and produces a run of an output transition system such that the combined run always satisfies a set of $GR(k)$ properties. 
