# Supplementary material for: Adapting Behaviors via Reactive Synthesis
Source: arXiv:2105.13837 source file (2021-05-28)
Supplement: Supplementary file 4 [file OldAppendixProofLeftovers.tex]

\section{Proof leftovers}\label{sec:appLeftovers}

Now we can finally present, in Algo~\ref{algo:sym-weak-buchi}, the symbolic modification of the inductive procedure from Section~\ref{subsec:dfa-game}. The algorithm returns the system's winning region ($W$) and a memory-less winning strategy ($f^s$). %We naturally model regions, i.e. sets of states, by BDDs over $\I,\O$. A memory-less strategy is modeled by a BDD over $\I,\O,\I',\O$ that relate a state and an input to a possible output. That is, for such BDD $\sigma$, $\sigma(\inp_0,\out_0,\inp_1',\out_1')$ means that from state $(\inp_0,\out_0)$ and input $(\inp_1)$, if the input is legal, then the strategy responds with $\out_1$. 
For the simplicity of the construction, we construct a strategy that is not necessarily deterministic. That is, we allow several possible responses for given state and input, and require that a resulting play is winning for the system, regardless of the non-deterministic choices made during the play. 

The algorithm employs two sub-procedures. (1) $\mathit{reach}(\beta,W)$ receives a BDD of a closed downwards set of SCCs, $\beta$, and a BDD of target states $W\subseteq \beta$. The procedure solves reachability in the subgame $\beta$ and target set $W$ and thus outputs a pair $(W_1,f^s_1)$: $W_1$ is the winning region of the system, and $f^s_1$ is a memory-less winning strategy. 
(2) $\mathit{safe}(\beta,W)$ receives a BDD of a closed downwards set of SCCs, $\beta$, 
and a BDD of safe states $W\subseteq \beta$. The procedure solves safety in the subgame $\beta$ and safe region $W$ and thus outputs a pair $(W_2,f^s_2)$: $W_1$ is the wining region of the system, and $f^s_2$ is a memory-less winning strategy. 

Lines~\ref{line:terminal}-\ref{line:winning-terminal-states} form the induction basis. We identify the terminal states (line~\ref{line:terminal}), identify the winning terminal states - the accepting SCCs (line~\ref{line:winning-variable}), and compute a winning strategy from those SCCs - a strategy that merely finds a legal input, as we cannot leave a terminal SCC (line~\ref{line:winning-terminal-states}).

Lines~\ref{line:while-loop}-\ref{line:end-while} form the induction step. After identifying the winning states $W$ in the subgame $\beta$ along with a matching memory-less strategy $f^s$, we wish to extend $W$ and $f^s$ to $\mathit{pre}(\beta)$. The additional winning states are those from which we can reach $W$ (line~\ref{line:reach}), denoted $W_1$, and the added accepting states (say, $A$) from which can force staying in $A$ or reaching $W$ (line~\ref{line:safe}),\footnote{see Section~\ref{subsec:dfa-game} for an explanation why we can use safety-game to identify this set of states} denoted $W_2$. In line~\ref{line:extend-strategy}, we extend the winning strategy over $W_1$ and $W_2$. We extend $f^s$ to $W_1\setminus W$: a strategy to reach $W$ from which we apply $f^s$. In addition, we extend the strategy to new discovered states from $W_2$: we play a safety strategy, and if the play reaches $W$, we switch to the already constructed strategy $f^s$.
We further update the set of discovered winning states (line~\ref{line:extend-region}).

\begin{algorithm}[t!]
	\caption{Weak-B\"uchi winning strategy construction}
	\label{algo:sym-weak-buchi}
	\begin{algorithmic}[1]
	    
	    \Statex \textbf{input:} A weak B\"uchi game $((\I,\O,\theta_\I,\theta_\O,\rho_\I,\rho_\O),GF\mathit{(acc)})$ 
	    
	    %\State construct $\beta_\mathit{SCC},\beta_\mathit{ter}$
	    
	    \State $\beta = \beta_\mathit{ter}$\label{line:terminal}
	    
	    \State $W=\beta\wedge \mathit{acc}$\label{line:winning-variable}
	    
	    \State $\sigma = W\wedge (\rho_\I\rightarrow \rho_\O)$\label{line:winning-terminal-states}
    
        \While{$\beta \neq 2^{\I\cup\O}$}\label{line:while-loop}
        
        \State $\gamma =\mathit{pre}(\beta)$\label{line:pre}
        
        \State $(W_1,f^s_1)=\mathit{reach}(\gamma,W)$\label{line:reach}
        
        \State $(W_2,f^s_2)=\mathit{safe}(\gamma,W\vee (  (\gamma\setminus \beta)\wedge \mathit{acc}))$\label{line:safe}
        
        \State $f^s = f^s \vee 
        ( (W_1\setminus W) \wedge f^s_1) \vee 
        ( (W_2\setminus (W\vee W_1)) \wedge f^s_2)$\label{line:extend-strategy}
        
        \State $W=W\vee W_1 \vee W_2$\label{line:extend-region}
        
        \State $\beta= \gamma$
        
        \EndWhile\label{line:end-while}
		
		\State\Return $(W,f^s)$
	\end{algorithmic}
\end{algorithm}

We turn to prove Theorem~\ref{Thrm:WeakBuchi}.
\begin{proof}[proof of Theorem~\ref{Thrm:WeakBuchi}]
Algorithm~\ref{algo:sym-weak-buchi} symbolically implements the inductive procedure from Section~\ref{subsec:dfa-game}. Hence, it correctly identifies the system's winning region, and constructs a winning strategy. It remains to show that it performs $O(N)$ symbolic operations. First, by Lemmas~\ref{lem:beta_SCC},~\ref{lem:beta_ter}, $\beta_\mathit{ter}$ is constructed in $O(N)$ operations. Hence, it sufficient to show that each loop execution consumes $O(|\mathit{pre}(\beta)\setminus\beta|)$ operations.   

By Lemma~\ref{lem:pre-beta}, each execution of line~\ref{line:pre} consumes $O(1)$ operations. Therefore, to prove the required, we show that the sub procedures perform  $O(|\mathit{pre}(\beta)\setminus\beta|)$ operations. We start with $\mathit{reach}(\gamma, W)$. This sub-procedure performs the next fixed point computation: $Z_0=W$, and $Z_{i+1}=\mathit{pre}_s(Z_i)\cup Z_i$, where $\mathit{pre}_s(X)$ is the set of states from which the system can force reaching $X$ in a single step. Thus, $Z_0\subseteq Z_1\subseteq \cdots$, and the winning region is $Z_i$ that satisfies $Z_i=Z_{i+1}$. We refer the reader to~\cite[Chapter~20]{2001automata} for a comprehensive discussion. Now, at each step $j< i$, at least one state is added to $Z_{j}$ thus there are at most $|\gamma\setminus W|$ steps, each is performed in $O(1)$ operations. Furthermore, if $s\in \beta\setminus W$, then we never add $s$ to a set $Z_j$. This claim is argued is follows. If we add $s$ to some $Z_j$, then the system can force reaching $W$ from $s$, and then it can win w.r.t. the B\"uchi condition. This contradicts the fact that $W$ is the system's winning region w.r.t. the B\"uchi condition  in the subgame $\beta$. Hence, an upper bound of $O(|\gamma\setminus\beta|)$ operations is established. 

Similarly, write $U=W\vee (\gamma\setminus \beta)\wedge \mathit{acc})$. $\mathit{safe}(\gamma,U)$ performs the next fixed point computation: $Z_0=U$, and $Z_{i+1}=Z_i \cap \mathit{pre}_s(Z_i)$. Thus, $Z_0\supseteq Z_1\supseteq \cdots$, and the winning region is $Z_i$ that satisfies $Z_i=Z_{i+1}$. See~\cite[Chapter~20]{2001automata} for a comprehensive discussion. As before, at each step $j<i$ at least a single state is removed from $Z_j$ and hence, an upper bound of $O(U)$ steps hold. Furthermore, a state $s\in W$ is never removed from $U$. This claim is argued as follows. Take $s\in W$, and assume that $s\in Z_j\setminus Z_{j+1}$. Consequently, the system cannot win $\mathit{safe}(W)$ from $s$ in the subgame $\beta$. Hence, the environment has a strategy to reach $\beta\setminus W$ form $s$, from which it can win w.r.t. the B\"uchi objective, in contradiction to $s\in W$. Therefore, the computation terminates after at most $O( |(\gamma\setminus\beta) \wedge \mathit{acc}|)$ steps, and an upper bound of $O(|\gamma\setminus\beta|)$ operation is established, which completes the proof.\qed 
\end{proof}
