# Supplementary material for: Adapting Behaviors via Reactive Synthesis
Source: arXiv:2105.13837 source file (2021-05-28)
Supplement: Supplementary file 5 [file OldAppendixStrategy.tex]

\section{Strategy appendix}


\paragraph{Computing the Winning Region.}

We can finally describe the fixed-point computation to construct a BDD for the winning region in  a weak \Buchi game. 
Let $\Reachability_{(A,B)}(\X)$
%\gatodo{I suggest to change the notation so it would be clear that A and B are parameters and X are vars. e.g. $\mathit{A-Reachabilty_B(X)}$ } 
denote a BDD, generated by solving a reachability game, that takes as input a set of source states $A$ and target states $B$, and outputs those states in $A$ from which the system can guarantee to move into $B$. Furthermore, let $\FReachability_{(A,B)}(\X,\X')$ be a BDD for the corresponding strategy.  
Similarly, let $\Safety_{(A,B)}(\X)$ denote a BDD, generated by solving a safety game, that takes as input a set of source states $A$ and target states $B$, and outputs those states in $A$ from which the system can guarantee that all plays remain inside the set $B$. Let $\FSafety_{(A,B)}(\X,\X')$ be a BDD for the corresponding strategy.
Details can be found in ~\cite[Chapter~2]{2001automata}.

In Algorithm~\ref{alg:weak-buchi},\gatodo{1. I wrapped the algorithm so it will be easy to refer to it.\\
2. I like the fixed-point presentation but perhaps it is better to use begin-end{algorithmic} to save some space.} we construct a BDD $\winning$ for the system's winning region, and a BDD $\strategy$ for a memory-less winning strategy from $\winning$.   $\winning$ is constructed as the fixed point of a family of BDDs $\winningAux^i$, and $\strategy$ as the fixed point of a family of BDDs $\strategyAux^i$, where the construction follows the description we gave earlier.

%Then, let  $\winning(s)$ denote that state $s$ over $\I\cup\O$ is in the winning region. Then, $\winning$ is the fixed point of $\winningAux$ which is defined below, where the construction essentially follows the explicit algorithm:
\begin{algorithm}[t!]
\label{alg:weak-buchi}
\begin{description}
    \item{\textbf{Base Case.}} $\winningAux^0(\X) := \terminal(\X) \wedge \varphi(X)$ and
    $\C^0(\X) := \terminal(\X)$
    
    $\strategyAux^0(\X,\X')= \terminal(X)\wedge (\rho_\I\rightarrow\rho_\O)(X)$
    
    \item {\textbf{Inductive Step.}} Define:
    
    \begin{align*}\C^{i+1}(\X) := & \forall \X': \Reach(\X,\X') \rightarrow (\SCC(\X,\X') \vee \C^i(X'))\\
    N(X):= & (\C^{i+1}(X)\setminus \C^i(X))\wedge \neg\varphi(X)\\
    A(X):= & (\C^{i+1}(X)\setminus\C^i(X))\wedge \varphi(X)
    \end{align*}
    
    \begin{align*}
    \winningAux^{i+1}(\X) & :=        \winningAux^i(\X) \\
    & \vee \Reachability_{(N(X), \winningAux^i(\X))}(X) \\
    &  \vee  
    \Safety_{(A(X), A(X)\vee\winningAux^i(\X))}(X)
  %  &\vee (\C^{i+1}(\X)\wedge \neg \C^{i}(\X)\wedge\varphi(\X)))
    \end{align*}
    
     \begin{align*}
    \strategyAux^{i+1}(X,X') & := \strategyAux^i(X,X') \\
       & \vee (N(X)\wedge\FReachability_{(N(X), \winningAux^i(\X))}(X,X')) \\
    &  \vee  
    (A(X)\wedge \FSafety_{(A(X), A(X)\vee\winningAux^i(\X))}(X,X'))
    \end{align*}
  
\end{description}
    \caption{Weak Buchi winning memory-less strategy construction }
\end{algorithm}

To explain the construction, note that a state $s$ in $\C^{i+1}(\X)$ \lmttodo{What does $\C$ mean?} \gatodo{DC probably stands for `downwards-closed`. Let's add some sentence about it - it will help to understand }is winning in one of these cases:
(i) Every state in $\winningAux^i(\X)$ is also winning.  
(ii) $s\in \C^{i+1}(X)\setminus \C^i(X)$ is non-accepting, and the system can force the play into the region $\winningAux^i(\X)$ (this set of states can be obtained from $\Reachability_{(N(\X), \winningAux^i(\X))}(X)$). 
(iii) %state in   $\C^{i+1}(\X)$ is winning if 
$s\in \C^{i+1}(X)\setminus \C^i(X)$ is accepting, and 
the system can force all plays from $s$ to remain in $A(\X)\cup \winningAux^i(\X)$ (this set of states can be obtained from $\Safety_{(A(X), A(X)\vee\winningAux^i(\X))}(X)$). 

A similar reasoning goes for the strategy $\strategyAux^{i+1}(X,X')$ from $\winningAux^{i+1}(X)$: 
(i) If $s\in \winningAux^i$ we follw $\strategyAux^{i}$. 
(ii) if $s\in \C^{i+1}\setminus \C^i$ is non-accepting, we activate $\FReachability(N(\X), \winningAux^i(\X))$ until reaching $\winningAux^i$. 
(iii) %state in   $\C^{i+1}(\X)$ is winning if 
if $s\in \C^{i+1}\setminus \C^i$ is accepting, we activate  $\FSafety_{(A(X), A(X)\vee\winningAux^i(\X))}(X)$, and if the play traverses out of $A(X)$, we switch to $\strategyAux^i$.

Finally, we prove the following theorem.

\begin{theorem}\label{thm:weakbuchi}
Realizability and synthesis for weak \Buchi games can be done in $O(N)$ symbolic steps.
\end{theorem}

\paragraph{Proof Outline.\gatodo{up to here. To revise to include the strategy or give up and refer to appx. }}
The proposed construction symbolically implements the inductive procedure of the explicit algorithm. Hence, it correctly identifies the system's winning region. 
It remains to show that the algorithm performs $O(N)$ symbolic operations. First, of all, the constructions of $\SCC$ and $\terminal$ take $\O(N)$ symbolic operations collectively. It suffices to show that in the $i$-th induction step, solving the reachability and safety games  performs  $O(|\pre(\C^{i+1})\setminus\C^i|)$ operations. This can be proven by a careful analysis of the operations and the sizes of resulting BDDs using standard results on safety and reachability games. Details have been deferred to the Appendix\gatodo{this high-level description explains realizability check, but I think it fails to explain the strategy construction}.\qed 


\subsection{Symbolically Solving Separated-GR($k$) Games}\label{sec:symsol-appendix}

Having a symbolic strategy for weak \Buchi games, we can finally show how to symbolically solve realizability and synthesis for Separated-GR($k$)\lmttodo{Keep capitalization consistent} games, followed by a time complexity analysis.
Our construction mainly follows the framework described previously. Our current solution for $f_t$ is a strategy with memory $|\varphi|$, as we detail below.

\paragraph{Defining accepting states}

We are given a Separated-GR($k$) game structure $\GS = (\I,\O,\theta_\I,\theta_\O,\rho_\I,\rho_\O)$ and an assertion $\varphi=\bigwedge_{l=1}^k \varphi_l$, where  $\varphi_l  =
\bigwedge_{i=1}^{n_l} GF(a_{l,i}) \rightarrow \bigwedge_{j=1}^{m_l} GF(g_{l,j}))$. We first need to represent $\GS$ and $\varphi$ as BDDs.\gatodo{??} These symbolic representations are standard in common in the literature e.g. \cite{}. \dftodo{complete} Next, we describe the set of accepting states symbolically. That is, we provide a linear-time construction of a BDD that recognizes all accepting states.


% This section presents an algorithm to solve separated GR($k$) games when represented symbolically as in Definition~\ref{def:separatedGRk}. From Theorem~\ref{}, we know it trivially reduces to a weak B\"uchi game. The task, therefore, is to present an algorithm for weak B\"uchi games when presented symbolically. More specifically, we design a BDD based algorithm to solve a weak B\"uchi game $(\GS,\ltlG\ltlF \varphi)$ where the assertions in the game structure $\GS = (\I,\O,\theta_\I,\theta_\O,\rho_\I,\rho_\O)$ and the assertion $\varphi$ are given in the form of a BDDs.



We call a state in an accepting SCC an \textit{accepting state}. We next turn to show that all accepting states can be identified efficiently. \dftodo{move lemma to 6.2}

\begin{lemma}
A\gatodo{like in 6.1} BDD $\beta_\mathit{acc}$ over $\I,\O$ such that $\beta_\mathit{acc}(\inp,\out)$ if $(\inp,\out)$ is accepting, can be constructed in $O(|\varphi|+N)$ symbolic operations.
\end{lemma}
\begin{proof}
Consider the BDD $\beta_\mathit{SCC}$,\lmttodo{Should this be $\SCC(X, X')$? Unify notation.} constructed in $O(N)$ operations (see Lemma~\ref{lem:beta_SCC}). Take a component $\varphi_l= 
\bigwedge_{i=1}^{n_l} GF(a_{l,i}) \rightarrow \bigwedge_{j=1}^{m_l} GF(g_{l,j})$. First, we identify all states such that their SCC includes a $g_{j,l}$-state. For $j\in\{1,\dots,m_l\}$, let $\beta_{g_{l,j}}$ be a BDD over $\I,\O,\I',\O'$ such that $\beta_{g_{l,j}}(\inp_0,\out_0,\inp_1',\out_1')$ iff $\out_1\models g_{l,j}$. Hence, the BDD $\gamma_{l,j}$ over $\I,\O$, defined by $\exists \I',\O'(\beta_\mathit{SCC} \wedge \beta_{g_{l,j}})$, accepts a state $(\inp,\out)$ if its SCC includes a state $s\models g_{l,j}$.

Now, we focus on the assumptions. Similarly to the former case, for $i\in\{1,\dots,n_i\}$, let $\beta_{a_{l,j}}$ be a BDD over $\I,\O,\I',\O'$ such that $\beta_{a_{l,j}}(\inp_0,\out_0,\inp_1',\out_1')$ iff $\inp_1\models a_{l,i}$. Hence, the BDD $\alpha_{l,i}$ over $\I,\O$, defined by $\forall \I',\O'(\beta_\mathit{SCC}\rightarrow \neg\beta_{a_{l,i}})$,
accepts a state $(\inp,\out)$ if its SCC does not includes a state $s$ such that $s\models a_{l,j}$.

Therefore, the BDD $\beta_\mathit{acc}$ is constructed by $\bigwedge_{l=1}^k(  (\bigwedge_{j=1}^{m_l}\gamma_{l,j}) \vee (\bigvee_{i=1}^{n_l} \alpha_{l,i}))$ \lmttodo{Should this be $\neg \alpha_{l,i}$?}. The construction is performed by $O(|\varphi|+N)$ operations. \qed
\end{proof}


\paragraph{Constructing $f_{B}$.}

Let $acc$ be the assertion represented by $\beta_\mathit{acc}$. We construct $f_{B}$ as the winning strategy of the weak \Buchi game $(\GS, \ltlG \ltlF (\acc))$, following Section~\ref{sec:accepting-SCCs}.

\paragraph{Constructing $f_{\travel}$.}


  See Algorithm~\ref{algo:winning-strategy}. For the presentation of $f_{\travel}$ we arbitrarily order all guarantees that appear in our GR($k$) formula: ${\gar}_0,\dots,{\gar}_{m-1}$. For each guarantee $\gar_j$, we take a reachability strategy $f_{r(j)}$ that never leaves the SCC it is applied from. For the sake of presentation, we assume that if  $s\in S$, an SCC that includes no $\gar_j$-state, then $f_{r(j)}$ returns a distinguished value $\bot$. We equip $f_\travel$ with a memory variable $\mathit{mem}\in\{0,\dots,m-1\}$. $f_\travel(s,i)$ is computed as follows: for $\mathit{mem},\mathit{mem}+1,\dots$ we find the first $\mathit{mem}+j$ such that the SCC of $s$ includes a $\gar_j$ state, and   activates $f_{r(\mathit{mem}+j)}$ to reach such state (loop in line 1). If no guarantees can be satisfied in $S$, we just return an arbitrary output to stay in $S$ (line 6). We remark that we chose a loop-based algorithmic presentation for readability purposes. However, $f_\travel$ can be implemented by BDD operations (without the distinguished value $\bot$) with memory of size $m$. The construction of $f_\travel$ requires $O(|\varphi|N)$ symbolic BDD-operations as we need to construct $m$ reachability strategies (clearly, $m\leq |\varphi|$). 


\paragraph{Combining the strategies}

Finally, we interleave the strategies into a single strategy $f$ as described in Algorithm \ref{algo:winning-strategy}. Correctness follows from Lemma~\ref{lem:win} below.

%Overall, the strategy depicted in Algorithm~\ref{algo:winning-strategy} is constructed  in $O(|\varphi|N)$ symbolic operations.\dftodo{expand more}


  \begin{algorithm}[t!]
  	\caption{A winning strategy}
  	\label{algo:winning-strategy}
  	\begin{algorithmic}[1]
		
		\setcounter{ALG@line}{-1}
		
		\State \textbf{initialization:} construct $\beta_\mathit{SCC}$, $\gamma{=}\exists\O'(\beta)$  \quad\quad\quad\quad\quad\quad\quad\quad {//  see Lemma~\ref{lem:beta_SCC}} 
		\Statex
		\Statex{\begin{center}
  				/*\quad\quad  From state $s$ and input $\inp$ \quad\quad*/
 		\end{center}}
	
  	    %\State construct $\beta_\mathit{SCC}$ \quad\quad\quad\quad\quad\quad\quad\quad\quad\quad\quad\quad\quad {//  see Lemma~\ref{lem:beta_SCC}} 
	
  	    %\State $\gamma = \exists\O'(\beta)$ 
	    
  		\State if $\beta_\mathit{acc}(s)$ and $\gamma(s,\inp')$ \Return $f_\travel(s,\inp)$
		
  		\State \Return $f_B(s,\inp)$
  	\end{algorithmic}
  	
  	
  	\begin{algorithmic}[1]
		
		\Statex{\begin{center}
  				/*\quad\quad  Implementation of $f_\travel(s,i)$ \quad\quad*/
 		\end{center}}
	\setcounter{ALG@line}{-1}
	
	\State \textbf{initialization}: $\mathit{mem}\leftarrow 0$
  	    \For{$i=0$ to $m-1$}
	    
	    \State $\mathit{target}=\mathit{mem}+i \mod m$
	    
  	    \State $\out= f_{r(\mathit{target})}(s,i)$
  	    \State if $\out\neq \bot$ \Return $\out$ 
  		\EndFor
		\State \Return $\out$ such that $\beta_{\mathit{SCC}}(s,\inp',\out')$

  	\end{algorithmic}
  	
  	
  	
  	
  \end{algorithm}
  
\subsubsection{Proof of Correctness} \dftodo{this needs to be smooth}

We now prove the correctness of the construction presented in this section, and as a consequence Theorem~\ref{thm:main}.

\begin{lemma}\label{lem:win-appendix} \gatodo{1. We cannot give this lemma her since we haven't defined precisely the strategies it is about. 2. We need (somewhere) to prove the correctness of the $f$. Then, lemma 2 follows almost immediately- no need in the proof we give here.}
If a winning strategy $f_B$ exists for the weak \Buchi game $B = (\GS,\ltlG \ltlF(\acc))$, then $f$ is a winning strategy for the separated GR($k$) game $(\GS, \varphi)$.
\end{lemma}

\begin{proof}
Since $f_B$ has a winning strategy, then for every initial input $\inp_0 \models \theta_\I$ there is an initial output $\out_0 \models \theta_\O$ such that $(i_0,o_0)$ is in the winning region of $B$.
We will show that playing $f$ always keeps the play in the winning region of $B$, and therefore the play eventually converges to an accepting SCC $S$. Once this happens, following $f_\travel$ guarantees that $\varphi$ is satisfied.\dftodo{put in a separate lemma}

We know that as long as the play is in the winning region of $B$, following $f_B$ will keep it inside the winning region. Therefore, when we switch from $f_B$ to $f_\travel$ we must be inside the winning region and, by definition of $f$, in an accepting SCC $S$. By Corollary~\ref{cor:delay}, as long as we remain inside $S$, which is guaranteed by $f_\travel$, the play will remain in the winning region. Therefore, the only way that the play can leave the winning region is if, while the system is following $f_\travel$, the environment chooses an input that takes the play to a different, non-winning SCC. We now prove that this cannot happen.

Assume that from state $(\inp_0, \out_0)$ in the accepting SCC $S$, the system chooses output $\out_{-m}$ according to $f_\travel$ and the environment chooses input $\inp_n$ such that $(\inp_n, \out_{-m})$ is in a different SCC. Note that $(\inp_0, \out_0)$ is in the winning region, there is a path from $\inp_0$ to $\inp_n$ and there is a path from $\out_{-m}$ to $\out_0$ (since by construction $f_\travel$ remains in the same SCC in $G_\O$). Therefore, by Theorem~\ref{thm:delay} $(\inp_n, \out_{-m})$ is in the winning region as well. 
\qed
\end{proof}

% \begin{proof}
% Since $B$ has a winning strategy, then for every initial input $\inp_0 \models \theta_\I$ there is an initial output $\out_0 \models \theta_\O$ such that $(i_0,o_0)$ is in the winning region of $B$.
% We will show that playing $f$ always keeps the play in the winning region of $B$. Therefore, the play eventually converges to an accepting SCC $S$, and by following $f_\travel$ the GR($k$) winning condition is satisfied.\dftodo{put in a separate lemma}

% To see that, we use the delay property corollary (about the winning region). Therefore as long $f^s_{wb}$ is switched to $f^s_{\mathit{travel}}$ and $f^s_{\mathit{travel}}$ is being played, the system remains in the winning region.

% Now assume that the strategy switched to $f^s_{wb}$ from $f^s_{\mathit{travel}}$. Then we have a state $s$ in an accepting $SCC$, i.e. in the winning region of $f^s_{wb}$,\gatodo{I have no idea what is a winning region of a strategy. Perhaps you mean that $f^s_{wb}$ wins from $s$?} and we need to see that $f^s_{wb}(s,i)$ is in the winning region of $f^s_{wb}$ as well \dftodo{why isn't it obvious???}. For that we use the delay property lemma \dftodo{I don't think we need to use it again} to show that we are still in the winning region \dftodo{clean!!!}.

% For the other side, note that if $(i_0,o_0)$ is not in the winning region of $f^s_{wb}$, then an accepting SCC cannot be reached by the system. Thus, every SCC that is reached does not meet the GR($k$) conditions. 

% \qed
% \end{proof}

As a consequence of Lemma~\ref{lem:win}, we get the following theorem.

\begin{theorem}\label{thm:realiizability}\gatodo{we can't give it here}
Realizability for separated GR($k$) games can be reduced to realizability of weak \Buchi games.
\end{theorem}

\begin{proof}
Given a separated GR($k$) game, if the corresponding weak \Buchi game is realizable the winning strategy $f_B$ can be used to compute $f$. If it is not realizable, then the environment can force every play to converge to a non-accepting SCC. Since the GR($k$) winning condition cannot be satisfied from a non-accepting SCC, the separated GR($k$) game is also not realizable.
% Given separated GR($k$) games $G$, construct the weak \Buchi game $G'$ by constructing the $\nu_{acc}$..
% Then check realizability for $G'$. By Lemma~\ref{lem:win}, we have that $G$ is realizable if and only if the initial state $(i_0,o_0)$ is in the winning region of a strategy for $G'$, i.e. iff $G'$ is realizable.
\qed
\end{proof}

We now use the reduction to weak \Buchi games in order to prove Theorem~\ref{thm:main}.

\paragraph{Proof of Theorem~\ref{thm:main}.}

Let GS be a game....



%  \subsection{Synthesizing a Winning Strategy}\label{sec:syntstrat}

%  We are ready to present a solution to the realizability and synthesis problem. We construct two strategies, each is constructed by $O(N)$ symbolic operations:
%  \begin{description}
%  \item[$f^s_{wb}$.] A memory-less strategy that wins the weak-B\"uchi game  $((\I,\O,\theta_\I,\theta_\O,\rho_{\I},\rho_{\O}),GF(\beta_{\mathit{acc}}))$.

%  \item[$f^s_{\mathit{travel}}$.] a memory-less strategy for the system to reach all possible inputs in a given SCC. That is, $f^s_\mathit{travel}$ satisfies the next property. Let $S$ be an SCC, and consider the subgame induced by $S$. Then, for every $(\inp,\out)\in S$, when the system applies $f^s_\mathit{travel}$, the play will traverse infinitely often states of the form $(\widehat{\inp},\out)$. \gatodo{I wonder how to construct such a strategy, symbolically, in $O(N)$ steps.}
%  \end{description}

%  Let $W$ be a winning region of $f^s_{wb}$. In Algorithm~\ref{algo:winning-strategy}, we present a strategy that wins for the system from $W$.




%  \begin{algorithm}[t]
%  	\caption{A winning strategy}
%  	\label{algo:winning-strategy}
%  	\begin{algorithmic}[1]
		
%  		\Statex{\begin{center}
%  				/*\quad\quad  From state $s$ and input $\inp$ \quad\quad*/
% 		\end{center}}
	
%  	    \State construct $\beta_\mathit{SCC}$ \quad\quad\quad\quad\quad\quad\quad\quad\quad\quad\quad\quad\quad {//  see Lemma~\ref{lem:beta_SCC}} 
	
%  	    \State $\gamma = \exists\O'(\beta)$ 
	    
%  		\State if $\beta_\mathit{acc}(s)$ and $\gamma(s,\inp')$ \Return $f^s_\mathit{travel}(s,\inp)$
		
%  		\State \Return $f^s_\mathit{wb}(s,\inp)$
%  	\end{algorithmic}
%  \end{algorithm}

%  We can now prove Theorem~\ref{thm:win}.
%  \begin{proof}
%  We show that $W$ is the system's winning region, and further that Algorithm~\ref{algo:winning-strategy} correctly constructs a strategy that wins from $W$.

%  First, we prove that Algorithm~\ref{} construct a strategy that wins from $W$. ...

% \end{proof}

\vspace{50mm}

********************Maybe:

After proving the delay property, it remains to describe how to construct the winning strategy. 
Given a separated GR($k$) game $(\GS, \varphi)$, we first find all accepting SCCs, and denote their union by $V_{acc}$. Let $\nu_{acc}$ be the assertion that accepts exactly those states in $V_{acc}$. Next, we construct the following:
\begin{description}
\item[$f_B$:] A memory-less strategy that wins the weak \Buchi game  $(\GS,\ltlG \ltlF(\nu_{acc}))$. An explicit algorithm that solves weak \Buchi games is described in~\cite{Chatterjee08}, and is given in Appendix~\ref{}\gatodo{we don't give it, right?}. In section~\ref{sec:accepting-SCCs} we describe in detail a symbolic algorithm.
Note that $f_B$ is \textit{not} the strategy constructed in the delay-property lemma.\gatodo{redundant, I think. We say that it is memory-less and we added a comment in the proof. }\lmttodo{I agree with Gal. Furthermore, at this point the reader doesn't know what strategy we are talking about, since the delay lemma hasn't been proved yet.}

\item[$f_\travel$:] A strategy for the system that, when played inside of an SCC $S_\O$ in $G_\O$, (a) always remains inside $S_\O$, and (b) for every guarantee $g_{l,j}$ in $\varphi$, visits a state that satisfies $g_{l,j}$ infinitely often as long as such a state exists in $S_\O$. Note that such a strategy always exists and can entirely ignore the inputs. Since the system can move in $G_\O$ regardless of the moves that the environment makes in $G_\I$, constructing $f_\travel$ can be done by simply finding a path in $S_\O$ that satisfies the maximum number of guarantees. We show this construction in Section~\ref{sec:symsol}. \dftodo{please clean this}
%A memory-less strategy for the system that reaches every state in a given SCC infinitely often. \dftodo{perhaps be more precise} \gatodo{I wonder how to construct such a strategy, symbolically, in $O(N)$ steps.}
\end{description}

Finally, we construct $f$, a strategy that combines $f_B$ and $f_\travel$ as follows: given a state $s$ and an input $i$, if $s$ is in an accepting SCC, apply $f_\travel$; else apply $f_B$. The strategy $f$ is a winning strategy for the separated GR($k$) game. We construct $f$ and prove its correctness in Section~\ref{sec:symsol} as well.

\begin{figure}[t]
    \centering
    \begin{subfigure}{0.33\textwidth}
        \centering
        \includegraphics[width=\textwidth,angle=-90]{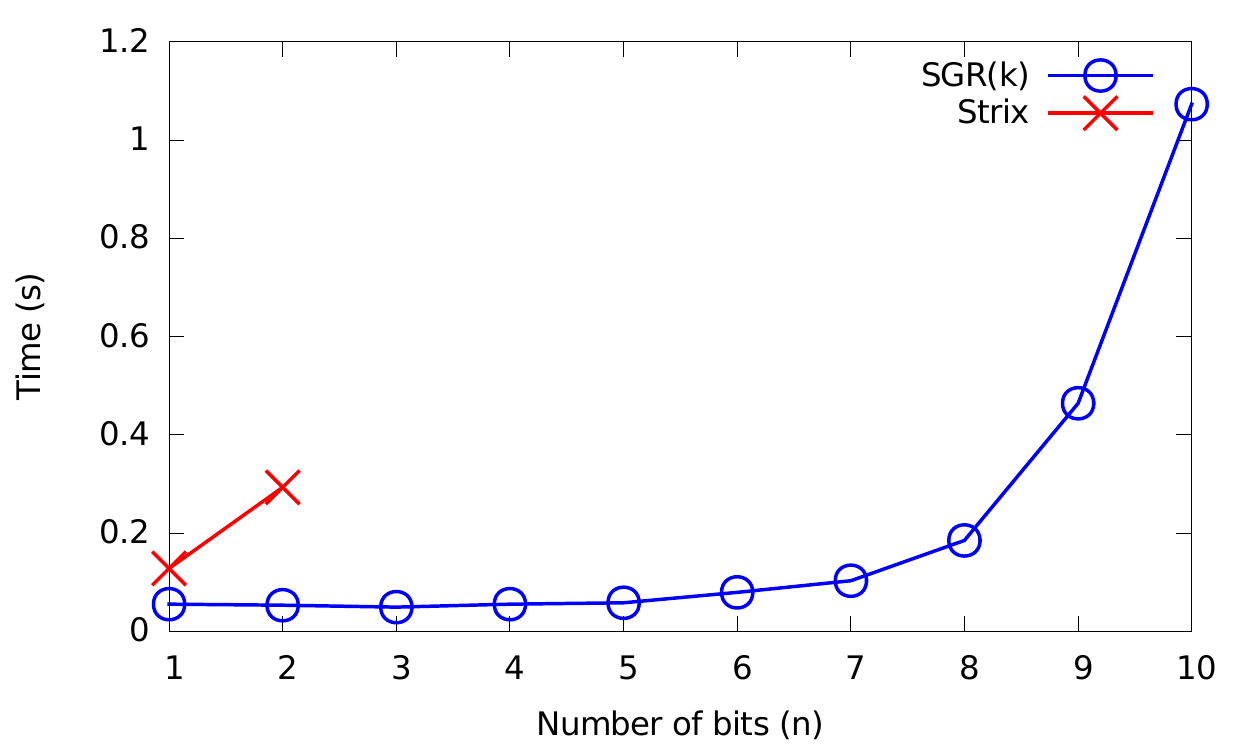}
        \caption{Motivating Example}
         \label{fig:cleaning-robots}
    \end{subfigure}%
    \hfill 
    \begin{subfigure}{0.33\textwidth}
        \centering
        \includegraphics[width=\textwidth,angle=-90]{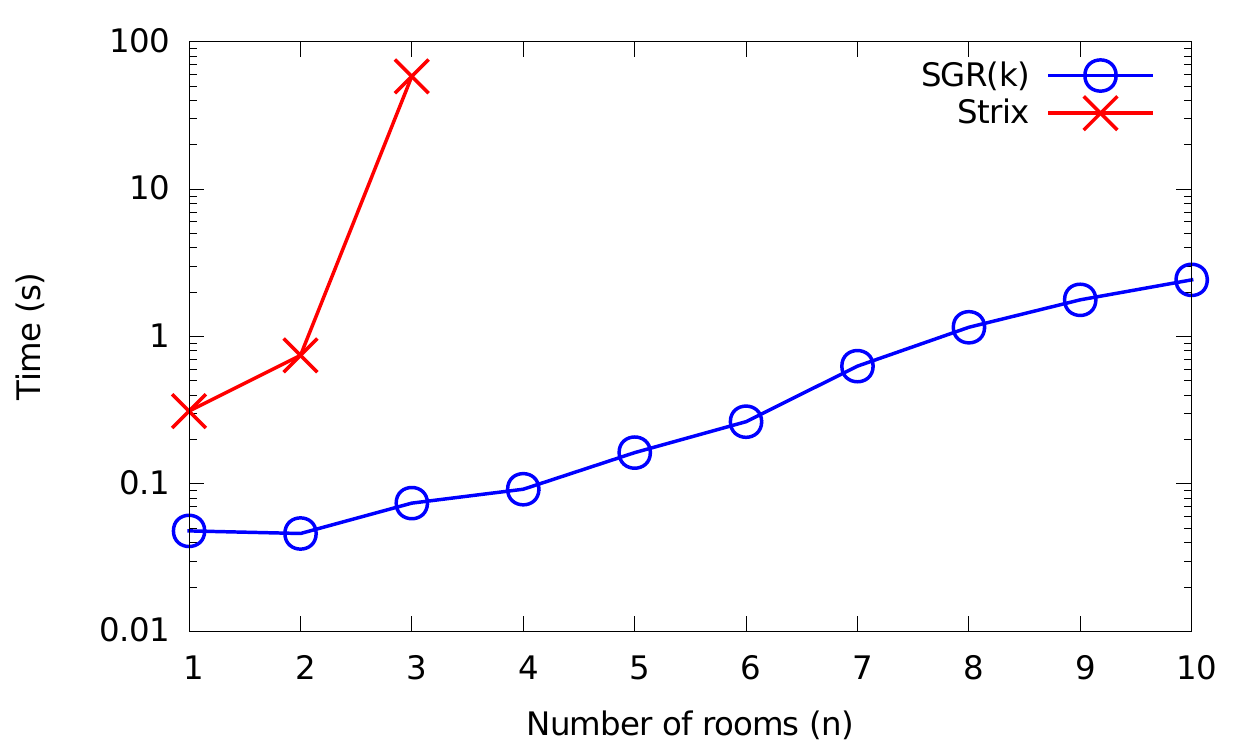}
        \caption{Cleaning Robots} 
    \end{subfigure}
    \hfill
    \begin{subfigure}{0.33\textwidth}
        \centering
        \includegraphics[width=\textwidth,angle=-90]{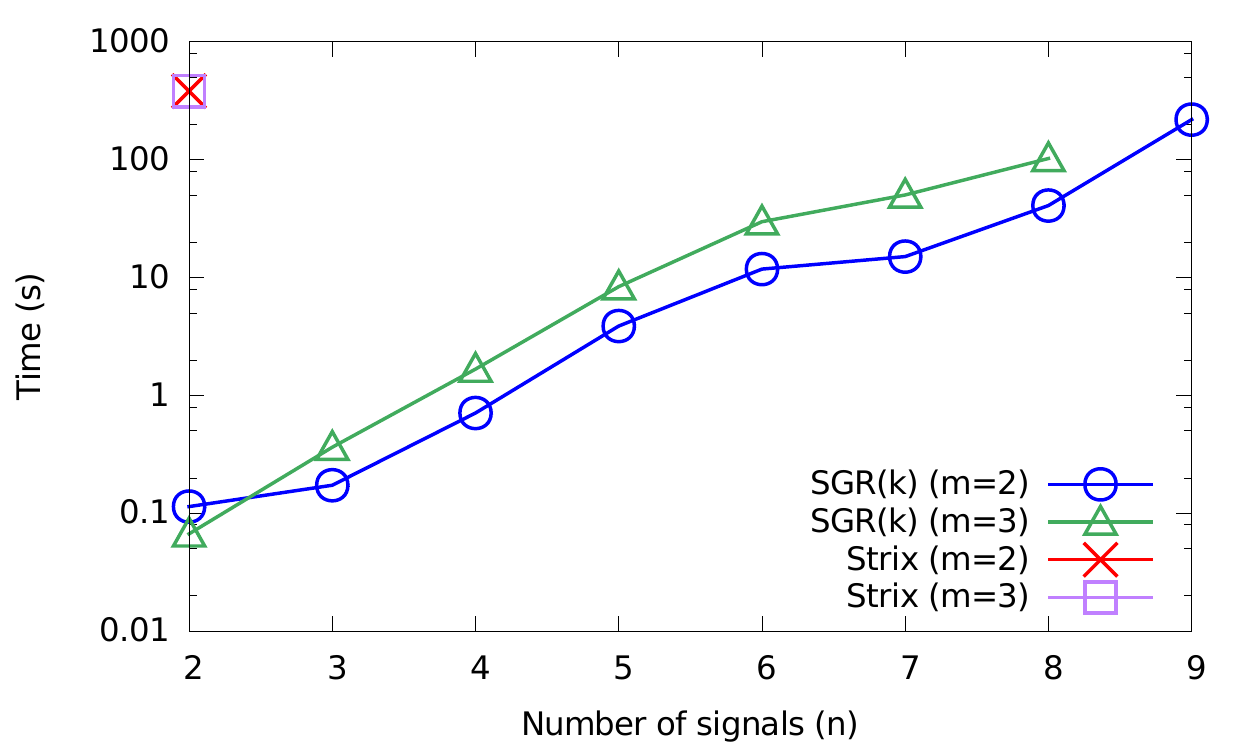}
         \caption{Railway Signalling}
         \label{fig:railway-signaling}
    \end{subfigure}
        \caption{Median running time for each class of benchmark.}
        \label{fig:running-time}
\end{figure}
