# Supplementary material for: Adapting Behaviors via Reactive Synthesis
Source: arXiv:2105.13837 source file (2021-05-28)
Supplement: Supplementary file 6 [file OldAppendixSym.tex]

\section{Details of the symbolic construction}
\label{app:symbCon}


In this section we describe how to implement the framework of Section~\ref{sec:delay} to solve realizability and synthesis for separated GR($k$) games. We describe our symbolic construction, follows by a complexity analysis.
Following our framework, we start by describing a symbolic construction of a strategy $f^{sym}_B$ that wins weak \Buchi games. Then we explain how to construct an overall strategy. Since our construction is BDD-based, we refer the reader to the appendix for the fine technical details.







Following our central result of  reduction of separated GR($k$) games to weak B\"uchi games presented in Section~\ref{sec:reduction}, this section presents a complete algorithm to solve separated GR($k$) games. By now, we know that the algorithm involves two steps: First, to obtain a weak B\"uchi game from the input separated GR($k$) by identifying  the SCCs. Second, to solve the resulting weak B\"uchi game. Since the input separated GR($k$) game is represented symbolically, the central requirement of our algorithm is to solve the above two steps symbolically. 
To this end, this section begins with an algorithm for separated GR($k$) games when they are  represented in an explicit-state representation in Section~\ref{sec:explicitweakbuchi}. 
%To this end, we begin with this sections begins by reviewing a linear-time algorithm to solve weak B\"uchi games when represented with explicit states in Section~\ref{sec:explicitweakbuchi}. 
Later, Section~\ref{sec:symbolicweakbuchi} will adapt the explicit-state algorithm to the desired symbolic state representation. 




%A \textit{subgraph} $G_0$ of a directed graph $G=(V,E)$ is a graph $(V_0,E_0)$ where $V_0\subseteq V$ and $E_0= E\cap (V_0\times V_0)$. 
%\textit{A path} in a graph $G=(V,E)$ is a sequence $(v_0,\cdots v_i)$ such that for all $0\leq j<i$, $(v_j,v_{j+1})\in V$. Note that a single vertex is also considered as a path.
%A \textit{strongly connected component} (SCC) in a graph $G=(V,E)$, is a maximal subset $V_0\subseteq V$ such that for every vertices $v,v' \in V_0$, there exists a path from $v$ to $v'$ in $G$. Note that the set of all SCCs forms a partition of the graph-vertices.
%An SCC, $S$ is a \emph{terminal SCC} if for every $s\in S$ the next holds: if a state $t$ is reachable from $s$, then $t\in S$.

%We exploit the special structure of the weak B\"uchi automaton to solve this game more efficiently than a typical Parity game or B\"uchi game. 


\subsubsection{Algorithm in explicit-state representation.} 

For sake of exposition, we present the algorithm when the separated GR($k$) game is represented explicitly. We observe that the algorithm is only {\em linear} in the size of the game when it is represented explicitly. 

Given a separated GR($k$) game $(\GS, \psi)$, we have already proven that the weak B\"uchi game over $(\GS, \ltlG\ltlF\varphi)$ where $\ltlG\ltlF\varphi= $ is such that the two games are equirealizable (Section~\ref{}). 
Let the separated GR($k$) game be explicitly represented over the directed game $(V,E)$. Then, in this section, we prove that separated GR($k$) game over directed graph $G = (V,E)$ is solved in $\O(|V|+|E|)$.

The first step is to generate the underlying weak B\"uchi game on $G=(V,E)$. The SCCs of $G$ can be identified in  $\O (|V|+|E|)$ time using the standard DFS-based algorithm. The challenge, however, is to identify which of these SCCs are accepting and which are non-accepting. 
The naive approach would be to generate the set $\F$ from $\varphi$, where $\ltlG\ltlF\varphi$ is the winning condition of the weak B\"uchi game, and determine whether $S_i\cap \F = \emptyset$ or $S_i\subseteq \F$ for every SCC $S_i$. This step is, however, expensive as the construction of $\F$ is exponential in the number of variables in $\I\cup\O$. 
To this end, we observe that a sufficient condition for an SCC to be accepting or non-accepting is for any one of its states to be accepting or non-accepting, respectively. Thus, for each SCC $S_i$, choose any one state $s_i \in S_i$. Since $s_i$ also represents an assignment over the $\I\cup\O$, evaluate $s_i \models \varphi$.  
Then the SCC $S_i$ is accepting if $s_i \models \varphi$ and non-accepting, otherwise. Since there are at most $|V|$ SCCs in graph $G$, the complexity of this step is $\O (|V|)$ (assuming the evaluation of $s_i\models \varphi$ is a constant time operation). Therefore, we have identified all the accepting and non-accepting SCCs of $G = (V,E)$ in $\O (|V|+|E|)$ time.

The next step is to solve realizability and synthesis on the weak B\"uchi game generated in the previous step. For this we use an exisiting linear-time algorithm for weak B\"uchi games~\cite{Chatterjee08}. For sake of completeness, we review the algorithm here:

\begin{theorem}[\cite{Chatterjee08}]
\label{Thrm:WeakBuchi}
Let a weak B\"uchi game be explicitly defined over directed graph $G = (V, E)$ with winning condition $\ltlG\ltlF\varphi$ where $\varphi$ is an assertion over input variables $\I$ and output variables $\O$ . 
The realizability and synthesis of the weak B\"uchi game are solved $\O(|V|+|E|)$ time. 
\end{theorem}

\paragraph{Algorithm description.}
We are given a weak B\"uchi game over $(V,E)$ with winning condition $\ltlG\ltlF\varphi$ in explicit state representation. As described earlier, the accepting and non-accepting SCCs can be identified in $\O(|V| + |E|)$.


Let $\Statess_0, \dots \Statess_m$ be the SCCs partitioning the directed graph $(V,E)$. W.l.o.g.,  let $\Statess_1>\Statess_2>\dots >\Statess_m$ with respect to the partial order $>$ induced by the topological sorting of the SCCs. 



\begin{description}
    \item[Base case:] %\gatodo{currently, the inductive process constructs the winning region. We also need to construct a memory-less strategy. A minor modification is needed for that...}
    $\Statess_m$ is a {\em terminal partition}, i.e., are no outgoing edges from $\Statess_m$. 
    
    By definition, plays beginning in any state of $\Statess_m$  will never leave it and be of infinite length. 
    Thus, if $\Statess_m$ is an accepting component, every state is a winning state for the system, while if $\Statess_m$ is a non-accepting component every state is a winning state for the environment.
    
    \item[Induction step:]
    Suppose all states in 
    $\Statess_{i+1}, \ldots, \Statess_m$ have been classified as winning for the system and environment, we determine which states in $\Statess_i$ are winning for each player.
    Due to the DAG-like structure induced by SCCs, the states in $\Statess_{i+1}$ to $\Statess_m$
    can be collapsed into two sink states, one winning for the system and the other winning for the environment. Then, all states in $\Statess_i$ can only reach other states in $\Statess_i$ or one of the two sink states. 
    
    Suppose, $\Statess_i$ is an accepting component. 
    Then, a state in $\Statess_i$ is winning for the system if it can either force plays to stay inside $\Statess_i$, or force the play to reach the accepting sink. 
    Alternately, a state is losing for the system if the environment can force plays into the losing sink. The losing states for the system can, thus, be computed by playing a reachability game with the losing sink as the reachability objective. Due to determinacy, the remaining states in $\Statess_i$ will be winning for the system. The strategy for the system from these winning states would be the one that enables it to remain inside these newly discovered winning states of go to the accepting sink.  
    
    %\gatodo{Since we also aim to construct a strategy, and not just to identify the winning region, it makes things simpler if we analyse the case (also) from the system perspective. We can add e.g.: Hence, in the accepting partition case, the system wins from its winning region w.r.t. $\mathit{safe}(Q_i\cup W)$, where $W$ are the winning states identified so far. Note that the system player can apply the following memory-less strategy. Play to win w.r.t. $\mathit{safe}(Q_i\cup W)$. If the play reaches $W$, apply the memory-less strategy from $W$.}
    
    Suppose, $\Statess_i$ is a non-accepting component. 
    Then, a state is winning for the system if it can force plays into the winning sink. 
    These states can be computed by playing a reachability game with the winning sink as the reachability objective. This will also determine the winning strategy for the system from these states.  
\end{description}

    Recall, reachability games can be solved in linear time. Thus, the complexity of the induction step on $\Statess_i$ is $\O(|\Statess_i|+|E_i|)$, where $E_i$ is the set of edges in $\Statess_i$. Furthermore, the identification of accepting and non-accepting SCCs and topological ordering of SCCs can be determined in $\O(|V|+|E|)$. 
    Thus, realizability and synthesis in weak B\"uchi games is solved in  $\O(|V|+|E|)$ where $(V,E)$ is the directed graph.

\begin{theorem}
\label{thrm:explicitalgorithm}
Realizability and synthesis on a separated GR($k$) game explicitly defined over a directed graph $G=(V,E)$ with winning condition $\psi$ is solved in $\O(|V|+|E|)$.
\end{theorem}
\begin{proof}
The proof is already present in the description of the two steps to solve separated GR($k$) games. Since each steps takes $\O(|V|+|E|)$ time to complete, the total complexity for synthesis and realizability is $\O(|V|+|E|)$.
\end{proof}

%There are a few interesting observations to weak B\"uchi games. First, note that not all states of an accepting partition are winning for the system and analogously not all states in a non-accepting partition are losing for the system. Note, additionally, that the algorithm described in Theorem~\ref{Thrm:WeakBuchi} necessarily need to be processed linearly. For example, if $Q_1$ only has transitions to $Q_3$ and $Q_4$, then the reachability game on $Q_1$ can be solved as soon as $Q_3$ and $Q_4$ are partitioned, even if $Q_2$ has not been partitioned yet. This allows for some degree of parallelism determined by the topology of the graph induced by the SCCs. In this case, for example, the reachability games for $Q_1$ and $Q_2$ could be solved in parallel. This may lead to significant speedups depending on the structure of the state space. \gatodo{I like the first observation. It helps the reader to see the full-picture. Not sure about the second... it is nice, but maybe too much... }

\begin{comment}
\subsubsection{Connected partition problem to weak B\"uchi games \gatodo{to omit?}}

We begin by describing the the connected partition problem under explicit state representation. 
Let $G$ be the product of the graphs $G_\I$ and $G_\O$, induced by the inputs $(I, \rho_\O)$ and $(\O,\rho_\O)$, as described in Section~\ref{Sec:graphdescription}. By abuse of notation, let $X$ also be an explicit state representation of the union of the SCCs. Then the winning condition for the system is $FG(X)$, i.e., the objective of the system is to  ensure that all plays of the game will eventually never leave the set $X$.
A state $q$ in the graph $G$ is said to be {\em winning for the system} if there exists a strategy for the system such that all plays beginning in $q$ 
satisfy the winning condition. A state $q$ is said to be {\em losing for the system} if for all strategies of the system, the environment can ensure that the winning condition is not satisfied.
Then, solving the connected partition problem is equivalent to determining whether there exist initial states of $G$ that are also winning states for the system.


The core insight of our solution is that the connected partition problem induces a weak B\"uchi game. 
To see how, recall that SCCs partition a graph and induce a DAG-like structure on it. Specifically, the graph $G$ can be interpret as a weak B\"uchi automaton as follows: Let $Q_1$,\dots $Q_m$ be the partitioning of the states of graph $G$ where every $Q_i$ is a distinct SCC. Then, due to the partitioning of the states in $G$ by SCCs, a partial order $>$ gets induced between the $Q_i$s due to the underlying DAG-like structure. In particular, for all $i$,$j$, $Q_i > Q_j$ if there exists a transition 
%Addressed. Having a transition is sufficient since if transiton exists then paths will also exist \gatodo{path, right?} 
from a state $q_i\in Q_i$ to state $q_j\in Q_j$.
Now, define the accepting states be the states in $X$. Since $X$ is a union of SCCs, by virtue of our assignment of accepting states, either all states in a given partition are accepting or all are non-accepting. Hence, the partitioning induced by the SCCs and assignment of states in $X$ as accepting, we obtain  a weak B\"uchi automaton. 
The connected partition problem is, therefore, equivalent to solving a game on a weak B\"uchi automaton in which the winning condition for the system is to eventually-globally visit its accepting states.

\begin{theorem}
\label{thrm:connectedpartitionexplicit}
In explicit state representation, the connected partition problem is solvable in linear time in size of the graph.
\end{theorem}
\begin{proof}
Each step of solving the connected partition problem, namely, computation of SCCs, topological sorting of the partitions, and solving the weak B\"uchi game are linear in the size of the underlying graph. Thus, connected partition problem is solved in linear time in size of the graph. 
\qed
\end{proof}

\end{comment}


\subsubsection{Symbolically identifying the accepting SCCs}
\label{sec:accepting-SCCs-appendix}

Since our algorithms are symbolic, we now turn to give a symbolic definitions of the weak \Buchi game and its components. While most of the symbolic representations are standard in common in the literature, we nevertheless describe below how to symbolically identify the accepting SCC. That is,  to provide a linear-time construction of a BDD that recognizes all accepting states.

% \begin{definition}
% Let $(\mathit{GS},\varphi)$ be a GR($k$) that separates variables, over the input/output variables, $\I$ and $\O$. Write $\varphi=\bigwedge_{l=1}^k \varphi_l$, where  $\varphi_l  =
% \bigwedge_{i=1}^{n_l} GF(a_{l,i}) \rightarrow \bigwedge_{j=1}^{m_l} GF(g_{l,j}))$. 
% Take a state $s\in 2^{\I\cup\O}$, and let $S$ be its SCC. Then, $s$ is accepting if for every $l\in\{1,\dots,k\}$ one of the following hold:
% \begin{description}
% \item[All guarantees hold in $S$.] For every $j\in\{1,\dots,m_l\}$, there exists $(\inp,\out)\in S$ such that $\out\models g_{l,j}$.

% \item[Some assumption cannot hold in $S$.] There exists $i\in\{1,\dots,n_l\}$ such that for all $(\inp,\out)\in S$, $\inp\not\models a_{l,i}$. 
% \end{description}
% \end{definition}

We first define every state in an accepting SCC as an \textit{accepting state}.
We next turn to show that all accepting states can be identified efficiently.

\begin{lemma}Let $(\mathit{GS},\varphi)$ be a GR($k$)-game that separates variables, over the input/output variables, $\I$ and $\O$. Write $\varphi=\bigwedge_{l=1}^k \varphi_l$, where  $\varphi_l  =
\bigwedge_{i=1}^{n_l} GF(a_{l,i}) \rightarrow \bigwedge_{j=1}^{m_l} GF(g_{l,j})
)$.
Then, a BDD $\beta_\mathit{acc}$ over $\I,\O$ such that $\beta_\mathit{acc}(\inp,\out)$ if $(\inp,\out)$ is accepting, can be constructed in $O(|\varphi|+N)$ symbolic operations.
\end{lemma}
\begin{proof}
Consider the BDD $\beta_\mathit{SCC}$, constructed in $O(N)$ operations (see Lemma~\ref{lem:beta_SCC}). Take a component $\varphi_l= 
\bigwedge_{i=1}^{n_l} GF(a_{l,i}) \rightarrow \bigwedge_{j=1}^{m_l} GF(g_{l,j})$. First, we identify all states that their SCC includes a $g_{j,l}$-state. For $j\in\{1,\dots,m_l\}$, let $\beta_{g_{l,j}}$ be a BDD over $\I,\O,\I',\O'$ such that $\beta_{g_{l,j}}(\inp_0,\out_0,\inp_1',\out_1')$ iff $\out_1\models g_{l,j}$. Hence, the BDD $\gamma_{l,j}$ over $\I,\O$, defined by $\exists \I',\O'(\beta_\mathit{SCC} \wedge \beta_{g_{l,j}})$, accepts a state $(\inp,\out)$ if its SCC includes a state $s\models g_{l,j}$.

Now, we focus on the assumptions. In similar to the former case, for $i\in\{1,\dots,n_i\}$, let $\beta_{a_{l,j}}$ be a BDD over $\I,\O,\I',\O'$ such that $\beta_{a_{l,j}}(\inp_0,\out_0,\inp_1',\out_1')$ iff $\inp_1\models a_{l,i}$. Hence, the BDD $\alpha_{l,i}$ over $\I,\O$, defined by $\forall \I',\O'(\beta_\mathit{SCC}\rightarrow \neg\beta_{a_{l,i}})$,
accepts a state $(\inp,\out)$ if its SCC does not includes a state $s$ such that $s\models a_{l,j}$.

Therefore, the BDD $\beta_\mathit{acc}$ is constructed by $\bigwedge_{l=1}^k(  (\bigwedge_{j=1}^{m_l}\gamma_{l,j}) \vee (\bigvee_{i=1}^{n_l} \alpha_{l,i}))$. The construction is performed by $O(|\varphi|+N)$ operations. \qed
\end{proof}






\subsection{Symbolic State Representation}
\label{sec:symbolicweakbuchi}

This section presents an algorithm to solve separated GR($k$) games when represented symbolically as in Definition~\ref{def:separatedGRk}. From Theorem~\ref{}, we know it trivially reduces to a weak B\"uchi game. The task, therefore, is to present an algorithm for weak B\"uchi games when presented symbolically. More specifically, we design a BDD based algorithm to solve a weak B\"uchi game $(\GS,\ltlG\ltlF \varphi)$ where the assertions in the game structure $\GS = (\I,\O,\theta_\I,\theta_\O,\rho_\I,\rho_\O)$ and the assertion $\varphi$ are given in the form of a BDDs. 

\subsubsection{Realizability}
To solve realizability, the goal is to compute a BDD for the winning region of the weak B\"uchi game and then to determine whether the initial states of the game intersects with the winning region. The construction of the winning region follows a fixed-point computation that adapts the inductive algorithm presented in  Section~\ref{sec:explicitweakbuchi}: In the basis of the fixed point computation, the winning region is the set of accepting and terminal SCCs; In the inductive step, the winning region includes winning states by examining SCCs that are higher in the topological ordering on SCCs. %There are several challenges in executing the fixed-point algorithm outlined here.  

% \newcommand{\SCC}{\mathsf{\mathsf{SCC}}}
% \newcommand{\Reach}{\mathsf{\mathsf{Reach}}}
% \newcommand{\Reachinverse}{\mathsf{\mathsf{Reach}^{-1}}}
% \newcommand{\Path}{\mathsf{\mathsf{Path}}}
% \newcommand{\terminal}{\mathsf{\mathsf{Terminal}}}
% \newcommand{\C}{\mathsf{\mathsf{DC}}}
% \newcommand{\pre}{\mathsf{\mathsf{pre}}}
% \newcommand{\winning}{\mathsf{\mathsf{Win}}}
% \newcommand{\winningAux}{\mathsf{\mathsf{Win\_Aux}}}
% \newcommand{\Reachability}{\mathsf{\mathsf{Reachability}}}
% \newcommand{\Safety}{\mathsf{\mathsf{Safety}}}



%\newcommand{\X}{\mathit{X}}
We begin with introducing necessary notation.
Let $B(\V)$ be a BDD defined over the ordered set of variables $\V = \{v_1, \ldots, v_n\}$. Let $W = \{w_1, \ldots, w_n\}$ be a new, ordered set of variables of the same cardinality. We use $B(W)$ to denote the BDD in which every variable $v_i$ is replaced with the corresponding variable $w_i$. We can extend this to a BDD $B(\V_1, \ldots, \V_m)$ over multiple sets $ \V_1, \ldots \V_m$ of variables in the natural way. 
Given an ordered set of variables $\V = \{v_1, \ldots, v_n\}$, we use $\V'$ to denote the ordered set of new variables $\V' = \{v'_1, \ldots, v'_n\}$.
We use the notation $\X$ to denote an ordered set of variables over $\I\cup\O$. 


\paragraph{BDD for SCCs.} We want to construct a predicate which indicates when two states in a game structure are present in the same SCC. Let us begin with predicate $\Reach(s,t')$ that holds if there is a path from state $s$ over $\I\cup\O$ to state $t$ over $\I\cup\O$ in the game structure $\GS$. Then, $\Reach$ is the fixed point computed iteratively as follows:


\begin{itemize}
    \item $\Path^{0}(\X, \X'):= (\I = \I') \wedge (\O = \O') $
    \item $\Path^{i+1} (\X,\X') := \exists  X'': (\rho_I\wedge \rho_O)(X,X'') \wedge \Path^{i} (X'',X')$
\end{itemize} 

Thus, a BDD for predicate  $\Reach$ is computed in $O(N)$ symbolic operations.
Similarly, let predicate 
$\Reachinverse(s,t')$ hold if there is a path from state $t$ over $\I\cup\O$ to state $s$ over $\I\cup\O$. Then  $\Reachinverse(s,t')$ holds iff $\Reach(t,s')$ holds. By a similar construction, a BDD for $\Reachinverse$ is constructed in $\O(N)$ symbolic operations. 

Then, define predicate $\SCC(s,t')$ to hold if states $s,t$ over $\I\cup\O$ are present in the same SCC in the game structure $\GS$. It is easy to see the following:  \[\SCC(\X,\X') := \Reach(\X,\X') \wedge \Reachinverse(\X,\X')\]

Therefore, a BDD for $\mathsf{SCC}$ is constructed in  $\O(N)$ symbolic operations. 




\paragraph{BDD for Terminal SCC.}
The induction basis for the construction of a winning region requires us to know what the terminal SCCs are. Let predicate $\terminal (s)$ hold if state $s$ over $\I\cup\O$ is present in a terminal SCC. Then
\[\terminal(\X) := \forall \X': \Reach(\X,\X')\rightarrow \SCC(\X,\X')
\]

Therefore, given BDDs for $\mathsf{Reach}$ and $\mathsf{SCC}$, the construction of $\mathsf{Terminal}$ requires $\O(1)$ symbolic operations. 

\paragraph{BDD to obtain SCCs higher in the topological ordering.}   
The induction step in the construction of the winning region requires us to know how to compute the {\em predecessor} SCCs w.r.t. to the topological ordering on the SCC.


Let $C$ be a set of SCCs over the game structure. For a state $s$ over $\I\cup\O$, let $s\models C$ be the shorthand for ``there exists an SCC $S\in C$ such that $s\models S $".
A set of SCCs $C$ is said to be {\em closed downwards} if for every state $s \models C$, for every state $t$ that is reachable from $s$, $t\models C$. If $C$ is closed downwards, then its predecessor, denoted $\mathit{pre}(C)\supseteq C$,  is  a set of SCCs  such that if $S$ is an SCC in $\mathit{pre}(C)$, states $s\models S$ and there exists a path from $s$ to  state $t$, then either $t\models S$ or $t\models C$. Note that $\mathit{pre}(C)$ is also closed downwards.
Observe that predicate $\terminal$ denotes a downward closed set of SCCs. 

Let predicate $\C$ over $\X$ denote a downward closed set of SCCs. Then, from the definition, we see that its predecessor $\pre(\C)$ can be obtained as follows:
\[
\pre(\C) := \forall \X': \Reach(\X,\X') \rightarrow (\SCC(\X,\X') \vee \C(X'))
\]

Then, a BDD for the predecessor of a $\pre(\C)$ is computed in $\O(1)$ symbolic operations, given a BDD for $\Reach$, $\SCC$, and the downward closed set $\C$.

\paragraph{Computing the Winning Region.}
Equipped with BDDs for $\SCC$, $\terminal$, and $\pre(\C)$ for a downward closed set of SCCs $\C$, we can finally describe the fixed-point computation to construct a BDD for the winning region in  a weak B\"uchi game. Recall, the game is defined over game structure $\GS=(\I,\O,\theta_\I,\theta_\O,\rho_\I,\rho_\O)$ and has a winning condition is given by $\ltlG\ltlF\varphi$. We assume, all assertions in $\GS$ and assertion $\varphi$ are given as a BDD in the input. 

Let $\Reachability(A,B)(\X)$ denote a BDD that takes as input a set of source states $A$ and target states $B$, and outputs those states in $A$ from which the system can guarantee to move into $B$. The BDD  for $\Reachability(A,B)$ is generated by solving a reachability game. Details can be found in ~\cite[Chapter~20]{2001automata}.


Let $\Safety(A,B)(\X)$ denote a BDD that takes as input a set of source states $A$ and target states $B$, and outputs those states in $A$ from which the system can guarantee that all plays remain inside the set $B$. $\Safety(A,B)(\X)$ is  generated by solving a safety game. 
Details can be found in ~\cite[Chapter~20]{2001automata}.


Then, let  $\winning(s)$ denote that state $s$ over $\I\cup\O$ is in the winning region. Then, $\winning$ is the fixed point of $\winningAux$ which is defined below. The construction essentially follows the algorithm presented in Section~\ref{sec:explicitweakbuchi}:
\begin{description}
    \item{\textbf{Base Case.}} $\winningAux^0(\X) := \terminal(\X) \wedge \varphi(X)$ and
    $\C^0(\X) := \terminal(\X)$
    
    \item {\textbf{Inductive Step.}} $\C^{i+1}(\X) := \pre(\C^i(\X))$.
    
    Then, a state in $\C^{i+1}(\X)$ is winning if the system can force to move into the region $\winningAux^i(\X)$. This set of states can be obtained from $\Reachability(\C^{i+1}(\X), \winningAux^i(\X))$. 
    
    Otherwise, a state in   $\C^{i+1}(\X)$ is winning if the system can force all plays in  $\C^{i+1}(\X)$ to remain in states in $A(\X) = \C^{i+1}(\X)\setminus\C^i(\X)$ that accept $\varphi$ or satisfy $\winningAux^i(\X)$. This set of states can be obtained from $\Safety(\C^{i+1}(\X), \winningAux^i(\X) \vee (\C^{i+1}(\X)\wedge \neg \C^{i}(\X)\wedge\varphi(\X)))$. 
    
    Finally, every state in $\winningAux^i(\X)$ is also winning.  Then, 
    \begin{align*}
    \winningAux^{i+1}(\X) & :=        \winningAux^i(\X) \\
    & \vee \Reachability(\C^{i+1}(\X), \winningAux^i(\X)) \\
    &  \vee  
    \Safety(\C^{i+1}(\X), \winningAux^i(\X) \vee (\C^{i+1}(\X)\wedge \neg \C^{i}(\X)\wedge\varphi(\X)))
    \end{align*}
  
\end{description}


Finally, we prove Theorem~\ref{Thrm:WeakBuchi}.
\begin{proof}[Proof Sketch of Theorem~\ref{Thrm:WeakBuchi}]
The proposed construction symbolically implements the inductive procedure from Section~\ref{sec:explicitweakbuchi}. Hence, it correctly identifies the system's winning region. 

It remains to show that the algorithm performs $O(N)$ symbolic operations. First, of all, the constructions of $\SCC$ and $\terminal$ take $\O(N)$ symbolic operations collectively. Give a downward closed set $\pre$ takes a $\O(1)$ symbolic operations. Hence, it sufficient to show that in the $i$-th induction step, solving the reachability and safety games  performs  $O(|\pre(\C^{i+1})\setminus\C^i|)$ operations. This can be proven by a careful analysis of the operations and the sizes of resulting BDDs using standard results on safety and reachability games. Details have been deferred to the Appendix.\qed 
\end{proof}

\subsubsection{Winning Strategy Extraction.} Since the algorithm solves reachability and safety games internally, the winning strategies of those games can be composed to generate a winning strategy to the weak B\"uchi game. Details have been deferred to the Appendix.

\begin{comment}
We are ready to modify the explicit strategy construction depicted in Section~\ref{subsec:dfa-game} into a symbolic one. The idea is to follow the outlined inductive procedure, while representing the relevant SCCs symbolically. 

We start with a technical construction that allows to replace variables with their primed version (or vice-versa).


Let $\beta$ be a BDD whose domain includes the the variable-sets $\V_1,\dots,\V_n$. We denote the BDD obtained from $\beta$ by replacing each $\V_i$ with $\V'_i$ by $R_{(\V_1\rightarrow\V_1',\dots,\V_n\rightarrow\V_n')}(\beta)$.
Our first goal is to show how to determine, symbolically, that two states belong to the same SCC.

\begin{lemma}
\label{lem:beta_SCC}
Let $\mathit{GS}= (\I,\O,\theta_\I,\theta_\O,\rho_\I,\rho_\O)$ be a game structure.  There exists a BDD $\beta_{\mathit{SCC}}$ over $\I,\O,\I',\O'$ such that $\beta_{\mathit{SCC}}(\inp_0,\out_0,\inp_1',\out_1')$ iff $(\inp_0,\out_0)$ and $(\inp_1,\out_1)$ belong to the same SCC. Moreover, $\beta_{\mathit{SCC}}$ can be computed in $O(N)$ symbolic operations. 
\end{lemma}

\begin{proof}
We construct a BDD $\beta_{\mathit{Reach}}$ over $\I,\O,\I',\O'$ such that $\beta_{\mathit{Reach}}(\inp_0,\out_0,\inp_1',\out_1')$ if there exists a path from $(\inp_0,\out_0)$ to $(\inp_1,\out_1)$ in $G^\mathit{GS}$. To this end, we repeatedly construct BDDs $\beta^0,\beta^1,\dots$ over $\I,\O,\I',\O'$ such that $\beta^i(\inp_0,\out_0,\inp_1,\out_1)$ if  there exists a path of length at most $i$ from $(\inp_0,\out_0)$ to $(\inp_1,\out_1)$. This process ends when $\beta^i = \beta^{i+1}$, and then we have $\beta_{\mathit{Reach}}=\beta^i$. Those are computed as follows:
\begin{itemize}
    
    \item $\beta^0$ is defined by $(\I=\I') \wedge (\O=\O')$.
    
    
    %\item $\beta^{i+1}(\inp_0,\out_0,\inp_1,\out_1) \Longleftrightarrow  (\exists \inp_2,\out_2\in \I\times\O\big( \beta^i(\inp_0,\out_0,\inp_2',\out_2') \wedge (\inp_2,\out_2,\inp_1',\out_1')\models (\rho_\I\wedge\rho_\O)\big))\vee \beta^i$.
    
    %\item To construct $\beta^1,\beta^2\dots$, we construct BDD $\rho$ over $\I',\O',\I'',\O''$ such that $\rho_{\mathit{copy}}(\inp_0',\out_0',\inp_1'',\out_1'')$ if $(\inp_0,\out_0',\inp_1',\out_1')\models \rho_\I\wedge \rho_\O$.
    
    %Now, Construct a BDD $\gamma^i$ over $\I',\O',\I'',\O''$ such that $\gamma(\inp_0',\out_0',\inp_1'',\out_1'')$ if $\beta(\inp_0,\out_0,\inp_1',\out_1')$. Construct a BDD $\delta^{i+1}$ over $??$ by   $\beta^i\wedge \I=\I''$ 
    
    \item $\beta^{i+1}$ is constructed as follows. Use replacement to construct a BDD $\rho$ over $\I,\O,\I'',\O''$ such that $\rho(\inp_0,\out_0,\inp_1'',\out_1'')\Longleftrightarrow (\inp_0,\out_0,\inp_1'\out_1')\models\rho_\I\wedge \rho_\O$. Construct a BDD $\gamma$ over $\I,\O,\I',\O',\I'',\O''$ by $\beta^i \wedge \rho$, and a BDD $\delta$ over $\I,\O,\I'',\O''$ by $\exists\I',\O'(\gamma)$. Note that $\delta(\inp_0,\out_0,\inp_1'',\out_1'')$ iff there exists a path from $(\inp_0,\out_0)$ to $(\inp_1,\out_1)$ of length $\l\in\{1,\dots,i+1\}$.
    Finally, $\beta^{i+1}$ is constructed by $R_{(\I''\rightarrow \I',\O''\rightarrow \O')}(\delta)\vee \beta^0$.
    
\end{itemize}

Hence, $\beta_{\mathit{Reach}}$ is computed in $O(N)$ symbolic operations. Likewise, we compute in $O(N)$ symbolic operations a BDD $\beta_{\mathit{Reach}^{-1}}$ over $\I,\O,\I',\O'$, satisfying $\beta_{\mathit{Reach}^{-1}}(\inp_0,\out_0,\inp_1',\out_1')$ if there exists a path in $G^\mathit{GS}$ from $(\inp_1,\out_1)$ to $(\inp_0,\out_0)$. Clearly, $\beta_{\mathit{SCC}} = \beta_{\mathit{Reach}} \wedge \beta_{\mathit{Reach}^{-1}}$.\qed
\end{proof}

To perform the induction basis, we identify all terminal SCCs in $O(1)$ symbolic operations.


\begin{lemma}
\label{lem:beta_ter}
Let $\mathit{GS}= (\I,\O,\theta_\I,\theta_\O,\rho_\I,\rho_\O)$ be a game structure.
Then, given the BDDs constructed above we can construct a BDD $\beta_{\mathit{ter}}$ over $\I,\O$ in $O(1)$ symbolic operations such that $\beta_{\mathit{ter}}(\inp,\out)$ iff $(\inp,\out)$ belongs to a terminal SCC.
\end{lemma}
\begin{proof}
During the construction of $\beta_{\mathit{SCC}}$, we constructed a BDD $\beta_{\mathit{Reach}}$ over $\I,\O,\I',\O'$ that satisfies $\beta_{\mathit{Reach}}(\inp_0,\out_0,\inp_1',\out_1')$ iff $(\inp_1,\out_1)$ is reachable from $(\inp_0,\out_0)$. Then, $\beta_{\mathit{ter}}$ is constructed by $\forall \I',\O' (\beta_\mathit{Reach}\rightarrow \beta_\mathit{SCC})$.\qed
\end{proof}





To apply the induction step our next goal is to compute the ``predecessor" SCCs of a downwards closed set of  SCCs.

\begin{definition}
Let $X$ be a set of SCCs.
\begin{enumerate}
    \item $X$ is closed downwards if for any $s\in X$, every state reachable from $s$ is also a member of $X$.
    
    \item If $X$ is closed downwards, then its predecessor is  a set of SCCs $\mathit{pre}(X)\supseteq X$  that satisfies: if $S\subseteq \mathit{pre}(X)$ is an SCC, $s\in S$, and there exists a path from $s$ to  state $t$, then $t\in S$ or $t\in X$. Note that $\mathit{pre}(X)$ is closed downwards.
\end{enumerate}\gatodo{Perhaps this def. should appear in the previous subsection}
\end{definition}



\begin{lemma}
\label{lem:pre-beta}
Let $\mathit{GS}= (\I,\O,\theta_\I,\theta_\O,\rho_\I,\rho_\O)$ be a game structure,
and $\beta$ be a BDD over $\I,\O$ that characterizes a closed downwards  set of SCCs, $X$.
Then, given the BDDs constructed above, a BDD $\mathit{pre}(\beta)$ for $\mathit{pre}(X)$ is computed in $O(1)$ symbolic operations.
\end{lemma}

\begin{proof}
Construct a BDD $\gamma$ by $R_{(\I\rightarrow \I', \O\rightarrow \O')}(\beta)$. Hence, $\mathit{pre}(\beta)$ is construct by $\forall \I',\O' (\beta_\mathit{Reach} \rightarrow (\beta_\mathit{SCC} \vee \gamma) )$.\qed
\end{proof}

Now we can finally present, in Algo~\ref{algo:sym-weak-buchi}, the symbolic modification of the inductive procedure from Section~\ref{subsec:dfa-game}. The algorithm returns the system's winning region ($W$) and a memory-less winning strategy ($f^s$). %We naturally model regions, i.e. sets of states, by BDDs over $\I,\O$. A memory-less strategy is modeled by a BDD over $\I,\O,\I',\O$ that relate a state and an input to a possible output. That is, for such BDD $\sigma$, $\sigma(\inp_0,\out_0,\inp_1',\out_1')$ means that from state $(\inp_0,\out_0)$ and input $(\inp_1)$, if the input is legal, then the strategy responds with $\out_1$. 
For the simplicity of the construction, we construct a strategy that is not necessarily deterministic. That is, we allow several possible responses for given state and input, and require that a resulting play is winning for the system, regardless of the non-deterministic choices made during the play. 

The algorithm employs two sub-procedures. (1) $\mathit{reach}(\beta,W)$ receives a BDD of a closed downwards set of SCCs, $\beta$, and a BDD of target states $W\subseteq \beta$. The procedure solves reachability in the subgame $\beta$ and target set $W$ and thus outputs a pair $(W_1,f^s_1)$: $W_1$ is the winning region of the system, and $f^s_1$ is a memory-less winning strategy. 
(2) $\mathit{safe}(\beta,W)$ receives a BDD of a closed downwards set of SCCs, $\beta$, 
and a BDD of safe states $W\subseteq \beta$. The procedure solves safety in the subgame $\beta$ and safe region $W$ and thus outputs a pair $(W_2,f^s_2)$: $W_1$ is the wining region of the system, and $f^s_2$ is a memory-less winning strategy. 

Lines~\ref{line:terminal}-\ref{line:winning-terminal-states} form the induction basis. We identify the terminal states (line~\ref{line:terminal}), identify the winning terminal states - the accepting SCCs (line~\ref{line:winning-variable}), and compute a winning strategy from those SCCs - a strategy that merely finds a legal input, as we cannot leave a terminal SCC (line~\ref{line:winning-terminal-states}).

Lines~\ref{line:while-loop}-\ref{line:end-while} form the induction step. After identifying the winning states $W$ in the subgame $\beta$ along with a matching memory-less strategy $f^s$, we wish to extend $W$ and $f^s$ to $\mathit{pre}(\beta)$. The additional winning states are those from which we can reach $W$ (line~\ref{line:reach}), denoted $W_1$, and the added accepting states (say, $A$) from which can force staying in $A$ or reaching $W$ (line~\ref{line:safe}),\footnote{see Section~\ref{subsec:dfa-game} for an explanation why we can use safety-game to identify this set of states} denoted $W_2$. In line~\ref{line:extend-strategy}, we extend the winning strategy over $W_1$ and $W_2$. We extend $f^s$ to $W_1\setminus W$: a strategy to reach $W$ from which we apply $f^s$. In addition, we extend the strategy to new discovered states from $W_2$: we play a safety strategy, and if the play reaches $W$, we switch to the already constructed strategy $f^s$.
We further update the set of discovered winning states (line~\ref{line:extend-region}).



\begin{algorithm}[t]
	\caption{Weak-B\"uchi winning strategy construction}
	\label{algo:sym-weak-buchi}
	\begin{algorithmic}[1]
	    
	    \Statex \textbf{input:} A weak B\"uchi game $((\I,\O,\theta_\I,\theta_\O,\rho_\I,\rho_\O),GF\mathit{(acc)})$ 
	    
	    %\State construct $\beta_\mathit{SCC},\beta_\mathit{ter}$
	    
	    \State $\beta = \beta_\mathit{ter}$\label{line:terminal}
	    
	    \State $W=\beta\wedge \mathit{acc}$\label{line:winning-variable}
	    
	    \State $\sigma = W\wedge (\rho_\I\rightarrow \rho_\O)$\label{line:winning-terminal-states}
    
        \While{$\beta \neq 2^{\I\cup\O}$}\label{line:while-loop}
        
        \State $\gamma =\mathit{pre}(\beta)$\label{line:pre}
        
        \State $(W_1,f^s_1)=\mathit{reach}(\gamma,W)$\label{line:reach}
        
        \State $(W_2,f^s_2)=\mathit{safe}(\gamma,W\vee (  (\gamma\setminus \beta)\wedge \mathit{acc}))$\label{line:safe}
        
        \State $f^s = f^s \vee 
        ( (W_1\setminus W) \wedge f^s_1) \vee 
        ( (W_2\setminus (W\vee W_1)) \wedge f^s_2)$\label{line:extend-strategy}
        
        \State $W=W\vee W_1 \vee W_2$\label{line:extend-region}
        
        \State $\beta= \gamma$
        
        \EndWhile\label{line:end-while}
		
		\State\Return $(W,f^s)$
	\end{algorithmic}
\end{algorithm}


We turn to prove Theorem~\ref{Thrm:WeakBuchi}.
\begin{proof}[proof of Theorem~\ref{Thrm:WeakBuchi}]
Algorithm~\ref{algo:sym-weak-buchi} symbolically implements the inductive procedure from Section~\ref{subsec:dfa-game}. Hence, it correctly identifies the system's winning region, and constructs a winning strategy. It remains to show that it performs $O(N)$ symbolic operations. First, by Lemmas~\ref{lem:beta_SCC},~\ref{lem:beta_ter}, $\beta_\mathit{ter}$ is constructed in $O(N)$ operations. Hence, it sufficient to show that each loop execution consumes $O(|\mathit{pre}(\beta)\setminus\beta|)$ operations.   

By Lemma~\ref{lem:pre-beta}, each execution of line~\ref{line:pre} consumes $O(1)$ operations. Therefore, to prove the required, we show that the sub procedures perform  $O(|\mathit{pre}(\beta)\setminus\beta|)$ operations. We start with $\mathit{reach}(\gamma, W)$. This sub-procedure performs the next fixed point computation: $Z_0=W$, and $Z_{i+1}=\mathit{pre}_s(Z_i)\cup Z_i$, where $\mathit{pre}_s(X)$ is the set of states from which the system can force reaching $X$ in a single step. Thus, $Z_0\subseteq Z_1\subseteq \cdots$, and the winning region is $Z_i$ that satisfies $Z_i=Z_{i+1}$. We refer the reader to~\cite[Chapter~20]{2001automata} for a comprehensive discussion. Now, at each step $j< i$, at least one state is added to $Z_{j}$ thus there are at most $|\gamma\setminus W|$ steps, each is performed in $O(1)$ operations. Furthermore, if $s\in \beta\setminus W$, then we never add $s$ to a set $Z_j$. This claim is argued is follows. If we add $s$ to some $Z_j$, then the system can force reaching $W$ from $s$, and then it can win w.r.t. the B\"uchi condition. This contradicts the fact that $W$ is the system's winning region w.r.t. the B\"uchi condition  in the subgame $\beta$. Hence, an upper bound of $O(|\gamma\setminus\beta|)$ operations is established. 

Similarly, write $U=W\vee (\gamma\setminus \beta)\wedge \mathit{acc})$. $\mathit{safe}(\gamma,U)$ performs the next fixed point computation: $Z_0=U$, and $Z_{i+1}=Z_i \cap \mathit{pre}_s(Z_i)$. Thus, $Z_0\supseteq Z_1\supseteq \cdots$, and the winning region is $Z_i$ that satisfies $Z_i=Z_{i+1}$. See~\cite[Chapter~20]{2001automata} for a comprehensive discussion. As before, at each step $j<i$ at least a single state is removed from $Z_j$ and hence, an upper bound of $O(U)$ steps hold. Furthermore, a state $s\in W$ is never removed from $U$. This claim is argued as follows. Take $s\in W$, and assume that $s\in Z_j\setminus Z_{j+1}$. Consequently, the system cannot win $\mathit{safe}(W)$ from $s$ in the subgame $\beta$. Hence, the environment has a strategy to reach $\beta\setminus W$ form $s$, from which it can win w.r.t. the B\"uchi objective, in contradiction to $s\in W$. Therefore, the computation terminates after at most $O( |(\gamma\setminus\beta) \wedge \mathit{acc}|)$ steps, and an upper bound of $O(|\gamma\setminus\beta|)$ operation is established, which completes the proof.\qed 
\end{proof}

\end{comment}




%%    commented out from here
\begin{comment}
\gatodo{I have few concerns about the weak-Buchi automata debate:\\
     {\large 1.} (somewhat minor) The advantages of mentioning weak-Buchi hare are clear - we want to prepare the reader for a (sort of) generalization of our solution to the connected-partition problem. The disadvantage is that we add "noise". More definitions that are distracting the reader, and may prevent her from understanding the solution to the connected partition problem. I wonder if the advantages justify the debate.\\
   {\large 2.} (somewhat minor) You gave the classical definition from the weak-Buchi paper. As Lucas noted, this def. is equivalent to: every SCC is either accepting or rejecting (right?) Wouldn't it be better to give that def.? It is simpler to grasp, and then there is no need to explain why the connected-partition problem is weak-Buchi.\\
   {\large 3.} (major) I disagree that connected-partition is a special case of Weak-Buchi. The problem is with the game rules. In the connected partition problem, the players choose the next state together: env chooses an input $\inp$, and sys chooses an output $\out$, and the play traverses to $(\inp,\out)$. In a weak-Buchi game, following standard definitions, the states are partitioned into player 0 and player 1 states. This is a huge difference. For example, it is possible that player i will play twice... Note that we can reduce the connected partition to weak Buchi as follows: we declare all states as env-states, and add "intermediate" sys-states of the form $(\inp_0,\out_0,\inp_1)$. This works but we do not benefit from it - We get a quadratic time complexity rather than linear. \\ \\
   My suggestion: I think it is better not to mention here weak-Buchi. Instead, in a spearte sect. to define a weak buchi game precisely and to mention that a straightforward adaptation of our algorithm works for weak-Buchi. Maybe we can even leave the proof for the reader/give it in an appx./ refer to an arxiv version that includes the proof.
}


\end{comment}

\begin{comment}
\subsection{Reduction to Finally-Globally (FG) winning condition}

Assume that each $\alpha_i$ and $\beta_i$ can be represented by a deterministic B\"{u}chi word automaton (DBW). Let $A_i$ be the the DBW for $\alpha_i$ and $B_i$ the DBW for $\beta_i$. Let $S_i$ be the set of states of $A_i$ and $T_i$ the set of states of $B_i$. Let $A = A_1 \times \ldots \times A_k$ be an automaton with state space $S = S_1 \times \ldots \times S_k$ and $B = B_1 \times \ldots \times B_k$ be an automaton with state space $T = T_1 \times \ldots \times T_k$. We say that a state $s = (s_1, \ldots, s_k)$ of $A$ is \emph{accepting for component $i$} if $s_i$ is an accepting state, and similarly for a state $t = (t_1, \ldots, t_k)$ of $B$.

For convenience, we assume that each player controls a single multi-valued variable, where each value corresponds to an assignment of the propositions controlled by that player. Let $x$ be the variable controlled by the environment, and $y$ the variable controlled by the system. We can write $A=(Q^A,\Sigma^A,q_0^A,\delta^A,F_1^A,\dots,F_k^A)$ and $B=(Q^B,\Sigma^B,q_0^B,\delta^B,F_1^B,\dots,F_k^B)$, where $\Sigma^A$ (resp. $\Sigma^B$) is the set of evaluations of $x$ (resp. $y$). For a word $w$ over $\Sigma^A$ (resp. $\Sigma^B$), $w\in L(\alpha_i)$ (resp. $w\in L(\beta_i)$) iff the run of $A$ (resp. $B$) on $w$ from $q_0^A$ (resp. $q_0^B$) traverses $F_i^A$ (resp. $F_i^B$) infinitely many times. 
 
We now define a game $D$ with $Q^A\times Q^B$ as the arena. From state $(q_i^A,q_j^B)$, the players choose together the ensuing state: the environment plays first, and it chooses a ``$\delta^A$-successor" of $q_i^A$, $q_{i'}^A$. In response, the system chooses a ``$\delta^B$-successor" of $q_j^B$, $q_{j'}^B$, and the ensuing state is $(q_{i'}^A,q_{i'}^B)$. A play is an infinite sequence of states, constructed according to the described procedure.\footnote{We assume that $A$ and $B$ are `complete', in the sense that $\mathit{Dom}(\delta^A)=Q^A\times \Sigma^A$ and $\mathit{Dom}(\delta^B)=Q^B\times \Sigma^B$.} 

Every trace in the original formula $\varphi$ can be lifted to a unique play in $D$ as follows. For a trace $(x_0,y_0),\dots,(x_m,y_m),\dots$, we take the play $(s_0^A,s_0^B),\dots ,(s_m^A,s_m^A),\dots$ where $(s_0^A,s_0^B)=(q_0^A,q_0^B)$ (the initial states), and $(s_{n+1}^A,s_{n+1}^B)=(\delta^A(s_n^A,x_n),\delta^B(s_n^B,y_n))$. Here, $x_n$ and $y_n$ are assignments to variables $x$ and $y$, respectively.

We say that a trace $\tau$ for $\varphi$ \emph{corresponds} to a play $\sigma$ in $D$, if $\tau$ is \emph{lifted} to $\sigma$, as described. Although $\tau$ corresponds to a unique play $\sigma$ in $D$, there are possibly many (yet, at least one) traces that correspond to a play $\sigma$ in $D$. The following observation is straightforward.

\begin{observation} \label{obs:streett}
If $\tau$ corresponds to $\sigma$, then $\tau$ satisfies $\varphi$ iff $\sigma$ satisfies the Streett condition: $(F_1^A,F_1^B),\dots,(F_k^A,F_k^B)$.
\end{observation}

\subsubsection{Defining a Winning Condition} \label{sec:fg-condition}

Following Observation~\ref{obs:streett}, we could solve the synthesis problem by solving a Streett game. In this section, however, we describe how we can simplify the winning condition to something of the form Finally-Globally (FG), which is easier to solve.

A state $q$ of $A$ (resp. of $B$) is an \emph{$i$-cycle} if there exists an $F_i^A$-state (resp. $F_i^B$-state) in its (strongly) connected component. A state $(q^A,q^B)$ of $D$ \emph{covers cycles} if for every $i\leq k$, if $q^A$ is an $i$-cycle, then $q^B$ is an $i$-cycle as well. Let $CC$ be the set of all states of $D$ that cover cycles.

We can also speak about connected component in $D$. Naturally, $(q^A,q^B)$ and $(q'^A,q'^B)$ are in the same connected component iff $q^A$ and $q'^A$ are in the same connected component in $A$, and $q^B$ and $q'^B$ are in the same connected component in $B$. Note that $CC$ is a property of a connected component. That is, $(q^A,q^B)\in CC$ iff all states in $(q^A,q^B)$'s connected component belong to $CC$.

Now, we turn to analyse the game $D$ w.r.t. the winning condition $FG(CC)$. Let $W_s$ and $W_e$ be the winning regions of the system and the environment in $D$ w.r.t. the winning condition $FG(CC)$, respectively. Standard determinacy arguments reveal that $W_s$ and $W_e$ partition the state space of $D$. 

\begin{lemma} \label{lemma:w_e}
$W_e$ is the set of states from which the environment has a strategy to force $FG(\overline{CC})$.
\end{lemma}
\begin{proof}
Let $\sigma=(p_0^A,p_0^A),\dots$ be a play in $D$. Since the play converges to a single connected component, we have $\sigma\models \neg FG(CC)\Longleftrightarrow \sigma\models FG(\overline{CC})$. Note that this proves a stronger property: it also proves that the a spoiling strategy for the environment w.r.t. the winning condition $FG(CC)$, also forces $FG(\overline{CC})$.
\end{proof}

\subsection{The Delay Property}

One of the crucial features of the game we have defined in this section is what we call the \emph{delay property}. Intuitively, this property says that the plays by the environment and the system need not be synchronized. That is, if a player can win from a state $(q^A, q^B)$, then the same player has a strategy to win even if the two players reach $q^A$ and $q^B$ at different times.
{\color{red} GaL: This is incorrect, the delay property means that the player can wait for awhile, letting the other player take several steps. For illustration, assume that sys has a strategy from $(q_A,q_B)$, sys reaches $q_B$ at time $t$, and at time $t+l$ the configuration is $(q_A,q_B')$. But, sys cannot win from $(q_A,q_B')$ (it is not difficult to construct such an example.) }

More formally, let $f_s : Q^A \times Q^B \rightarrow Q^B$ be a strategy for the system that wins from state $(q^A,q^B)$, and let $q'^B$ be a system state such that $\delta^B(q'^B,y_i)=q^B$ for some evaluation $y_i$ of $y$. Then, we can define a strategy $g_s : (Q^A \times Q^B) \times Q^A \rightarrow Q^B$ for the system that wins from state $(q^A, q'^B)$. This $g_s$ is a function from the current state $(p^A_1, p^B_1) \in Q^A \times Q^B$ and the previous environment state $p^A_0 \in Q^A$ to the next system state $p^B_2$. Note that, as $g_s$ needs to remember the previous environment state, it is not a memoryless strategy. 

Given $f_s$, $(q^A,q^B)$ and $q'^B$, we construct $g_s$ as follows. Assume that when we start from state $(q^A, q'^B)$ the previous environment state is $\epsilon$, indicating the lack of a predecessor. {\color{red} Gal: I don't understand the $\varepsilon$ here. But, It seems that it is not that important... } Then:
\begin{align*}
    &g_s((q^A, q'^B), \epsilon) = q^B \\
    &g_s((p^A, p^B), p'^A) = f(p'^A, p^B)
\end{align*}

Intuitively, $g_s$ first moves from $q'^B$ to $q^B$. Note that at this point the environment has also moved to another state $q'^A$. Afterwards, $g_s$ simply simulates $f_s$, but using the previous environment state instead of the current one. For example, after the game moves from $(q^A, q'^B)$ to $(q'^A, q^B)$, $g_s$ should make the same move from $(q'^A, q^B)$ as $f_s$ would make from $(q^A, q^B)$. In other words, after the first move, $g_s$ acts exactly like $f_s$, but with a delay of a single step.

The following lemma then follows directly from the definition of $g_s$:

\begin{lemma}
If $(p_0^A,p_0^B),\dots,(p_i^A,p_i^B)$ is a sequence from $(q^A,q'^B)$ that is consistent with $g_s$, then $(p_0^A,p_1^B),\dots, (p_{i-1}^A,p_i^B)$ is a sequence from $(q^A,q^B)$ that is consistent with $f_s$.
\end{lemma}

We now prove that $g_s$ is indeed a winning strategy from $(q^A, q'^B)$.

\begin{lemma}
$g_s$ is winning from $(q^A, q'^B)$.
\end{lemma}
\begin{proof}
Consider a play $\sigma_g=(p_0^A,p_0^B),\dots$ from $(q^A,q'^B)$, consistent with $g_s$. By the construction, $\sigma_f=(p_0^A,p_1^A),(p_1^A,p_2^B),\dots$ is a play, consistent with $f_s$, from $(q^A,q^B)$. Since $f_s$ is winning from $(q^A,q^B)$, $\sigma_f\models FG(CC)$. Therefore, after a finite amount of time $\sigma_f$ gets stuck in a $CC$ connected component. Since the environment and system states visited after this point in $\sigma_g$ are the same, $\sigma_g$ must get stuck in the same connected component. Hence, $g_s\models FG(CC)$.
\end{proof}

\begin{lemma} \label{lemma:delay}
The following hold.
\begin{itemize}

    
    \item[(1)] If $(q^A,q^B)\in W_s$ and $\delta^B(q'^B,y_i)=q^B$ for some evaluation of $y$, $y_i$, then $(q^A,q'^B)\in W_s$.
    
    \item[(2)] If $(q^A,q^B)\in W_e$ and $\delta^A(q'^A,x_i)=q^A$ for some evaluation of $x$, $x_i$, then $(q'^A,q^B)\in W^e$.
\end{itemize}

\end{lemma}
\begin{proof}
(1) follows directly from the construction of $g_s$ from $f_s$. For (2), we can invoke Lemma~\ref{lemma:w_e} to choose a strategy $f_e$ for the environment that forces $FG(\overline{CC})$. Then, with a similar construction we can get a strategy $g_e$ that forces $FG(\overline{CC})$ from $(q'^A, q^B)$.
\end{proof}

We can then obtain the following corollary by iterating Lemma~\ref{lemma:delay}.

\begin{corollary} The following hold.
\begin{itemize}
    \item[(1)] If $(q^A,q^B)\in W_s$ and $q^B$ is reachable in $B$ from $q'^B$, then $(q^A,q'^B)\in W_s$.
    
    \item[(2)] If $(q^A,q^B)\in W_e$ and $q^A$ is reachable in $A$ from $q'^A$, then $(q'^A,q^B)\in W_e$.
\end{itemize}
\end{corollary}

\begin{corollary} The following hold.
\begin{itemize}
    \item[(1)] If $(q^A,q^B)\in W_s$ and $q'^A$ is an $A$-successor of $q^A$, then $(q'^A,q^B)\in W_s$.
    
    \item[(2)] If $(q^A,q^B)\in W_e$ and $q'^B$ is a $B$-successor of $q^B$, then $(q^A,q'^B)\in W_e$.
\end{itemize}
\end{corollary}
\begin{proof}
To prove (1), take $(q^A,q^B)\in W_s$, and assume towards a contradiction that $(q'^A,q^B)\notin W_s$. Hence, $(q'^A,q^B)\in W_e$, and by the previous lemma $(q^A,q^B)\in W_e$ as well, in contradiction to the assumption. Claim (2) is implied by the same argument. 
\end{proof}

\subsection{Correctness of the Reduction}

We now prove the correctness of the reduction of the Streett winning condition from Observation~\ref{obs:streett} to the FG(CC) winning condition defined in Section~\ref{sec:fg-condition}.

Assume that $(q_A,q_B)\in W_s$, and let $f_s$ be a winning strategy for the system w.r.t. $FG(CC)$.\footnote{We can take a memoryless strategy $f^s$. Otherwise, some small technical changes are required.} Let $g_s:Q^B\rightarrow Q^B$ be a partial function such that:
\begin{enumerate}
    
    \item For each $q^B\in Q^B$, if $q^B$ has a successor in its connected component, then $g_s(q^B)$ is such a successor.
    
    \item Let $p_0^B,\dots,p_n^B,\dots$ be an infinite sequence over $Q^B$ such that for each $i$ $p_i^B=g^i(p_0^B)$. Thus, each state in $p_0^B$'s connected component appears in that sequence infinitely often.
\end{enumerate}
We set the following strategy $h_s$ for the system that is winning w.r.t. the Streett condition. From state $(q^A,q^B)$ and input $q'^A$:
\begin{itemize}
    \item If $(q'_A,q_B)\in CC$ and $g_s(q_B)$ is defined, then return $g_s(q^B)$.
    \item Otherwise, return $f_s((q^A,q^B),q'^A)$.
\end{itemize}

The following claim that the strategy is indeed well-defined
\begin{claim} \label{claim:h_s}
Take $(p_0^A,p_0^B)\in W_s$.
If $(p_0^A,p_0^B),\dots,(p_n^A,p_n^B)$ is consistent with $h_s$, and $p_{n+1}^A$ is an $A$-successor of $p_n^A$, then $h((p_n^A,p_n^B),p_{n+1}^A)$ is defined, and for $p_{n+1}^B=h((p_n^A,p_n^B),p_{n+1})$, it holds that $(p_{n+1}^A,p_{n+1}^B)\in W_s$. 
\end{claim}
\begin{proof}
We prove the claim by induction on $n$.
First, note that $(p_n^A,p_{n}^B)\in W^s$.
If $n=0$ this holds by assumption, and otherwise it holds by the induction hypothesis. Now, if $q_{n+1}^B$ is chosen according to the first item, then Corollaries 1 and 2 ensure that $(q_{n+1}^A,q_{n+1}^B)\in W_s$. Otherwise, $h$ returns $f_s((q_{n}^A,q_n^B),q_{n+1}^A)$. Since $(q_n^A,q_n^B)\in W_s$, $q_{n+1}^B$ is well-defined. Since the sequence $(q_{n}^A,q_n^B),(q_{n+1}^A,q_{n+1}^B)$ is consistent with $f_s$, $(q_{n+1}^A,q_{n+1}^B)\in W_s$, as required.
\end{proof}

We can now use the construction of $h_s$ to prove the following lemma.

\begin{lemma}
$(q^A,q^B)\in W_s$ iff the system player can win from $(q^A,q^B)$ w.r.t. the Streett condition $(F_1^A,F_1^B),\dots,(F_k^A,F_k^B)$. 
\end{lemma}

\begin{proof}
($\rightarrow$) Let $f_s$ be a winning strategy for the system w.r.t. $FG(CC)$ and construct $h_s$ as above. Now, we show that $h_s$ is winning w.r.t. the Streett condition. Take a play from $W_s$, $(p_0^A,p_0^B),\dots$ consistent with $h_s$. Hence, some suffix of the play, $(p_i^A,p_i^B),\dots$ never leaves a certain connected component. We consider two cases:
\begin{enumerate}
    \item The suffix stays in a $CC$-component. Then, at that suffix, $h_s$ consistently applies $g_s$ to choose the next output. It follows that the play satisfies the Streett condition.
    
    \item The suffix stays in a $\overline{CC}$-component. Then, at that suffix, $h_s$ consistently applies $f_s$ to provide the next output. Therefore, the play $(p_i^A,p_i^B),\dots$ is a losing play for the system w.r.t. $FG(CC)$, and it is consistent with $f_s$. Consequently, $(p_i^A,p_i^B)\notin W_s$. However, this conclusion contradicts Claim~\ref{claim:h_s} thus this case cannot occur. 
\end{enumerate}
As a result, it follows that $h_s$ is a winning strategy from $W_s$ w.r.t. the Streett condition $(F_1^A,F_1^B),\dots,(F_n^A,F_n^B)$, as required.

($\leftarrow$) We show that the environment has a spoiling strategy w.r.t. the street condition from $W_e$. Take a (memoryless) strategy for the environment $f_e$ from $W_e$, that forces $FG(\overline{CC})$. By Lemma~\ref{lemma:w_e}, such a strategy exists. Let $g_e:Q^A\rightarrow Q^A$ be a partial function that satisfies the analogous requirements as for $g_s$.  

We set the following strategy $h_e$ for the system. From state $(q^A,q^B)$:
\begin{itemize}
    \item If $(q_A,q_B)\in \overline{CC}$ and $g_e(q_A)$ is defined, then return $g_e(q^A)$.
    \item Otherwise, return $f_e((q^A,q^B))$.
\end{itemize}
By similar arguments as before, the claim follows.
\end{proof}

By the previous lemma, we have:
\begin{theorem} \label{thm:win}
System has a winning strategy iff $(q_0^A,q_0^B)\in W_s$. Such a strategy can be constructed from the strategy $h_s$.
\end{theorem}

\subsection{Solving the $FG(CC)$ Game}

Note that the $FG(CC)$ winning condition makes the game we have described a co-Büchi game where $CC$ is the set of accepting states. As noted in Section~\ref{sec:fg-condition}, $CC$ is a property of a connected component, meaning that for each connected component, either all states are in $CC$ or none are. This matches the definition of a weak automaton:

\begin{definition}
A co-Büchi automaton is said to be \emph{weak} if there is a partitioning of its state space $Q$ into $Q_1, \ldots, Q_m$ such that:

\begin{enumerate}
    \item For every $i$, either all states in $Q_i$ are accepting or all states are non-accepting.
    \item For every $i$ and $j$, if there exists a transition from state $q \in Q_i$ to state $q' \in Q_j$, then $i \leq j$.
\end{enumerate}
\end{definition}

$Q_1, \ldots, Q_m$ can be defined appropriately as the connected components of the state space, sorted topologically. Note that weak automata are more commonly defined with a Büchi acceptance condition, but since a play can never return to a previous connected component, Büchi and co-Büchi acceptance conditions are equivalent for weak automata.

We can therefore use the special properties of a weak automaton to solve this game more efficiently than a typical Büchi or co-Büchi game. A game over a weak automaton can be solved in linear time on the number of states:

\begin{description}
    \item[Base case:] Note that a play that reaches $Q_m$ cannot ever leave $Q_m$, since it is a terminal connected component. Therefore, if $Q_m$ is an accepting component every state is a winning state, while if $Q_m$ is a non-accepting component every state is a losing state.
    \item[Induction step:] If all states in $Q_{i+1}, \ldots, Q_m$ have been classified as winning or losing, they can be collapsed into two sink states, one winning and one losing. Then, all states in $Q_i$ can only reach other states in $Q_i$ or one of the two sink states. We can now partition the states in $Q_i$ into winning and losing states by solving a reachability game, where a state is winning if the game can be forced into the winning sink from it. Since reachability games can be solved in linear time, the complexity of this step is linear on $|Q_i|$.
\end{description}

Note, additionally, that the connected components do not necessarily need to be processed linearly. For example, if $Q_1$ only has transitions to $Q_3$ and $Q_4$, then the reachability game on $Q_1$ can be solved as soon as $Q_3$ and $Q_4$ are partitioned, even if $Q_2$ has not been partitioned yet. This allows for some degree of parallelism determined by the topology of the dependence graph between the connected components. In this case, for example, the reachability games for $Q_1$ and $Q_2$ could be solved in parallel. This may lead to significant speedups depending on the structure of the state space.

\end{comment}
